# Supplementary material for: Measuring Human Values in Text With Classifiers: Decision Rules, Bias, and Group Comparisons
Source: arXiv:2601.14172 ancillary file (2026-12-02)
Supplement: Supplementary file 1 [file paper-supplement.pdf]

# Supplementary Material for *Human Values in a Single Sentence: Moral Presence, Hierarchies, and Transformer Ensembles on the Schwartz Continuum*

Víctor Yeste[a,b,*], Paolo Rosso[a,c]

[a] *PRHLT Research Center, Universitat Politècnica de València, Valencia, 46022, Spain*
[b] *School of Science, Engineering and Design, Universidad Europea de Valencia, Valencia, 46010, Spain*
[c] *Valencian Graduate School and Research Network of Artificial Intelligence (ValgrAI),*

**Abstract**

This document contains supplementary material for the article *"Human Values in a Single Sentence: Moral Presence, Hierarchies, and Transformer Ensembles on the Schwartz Continuum"*. It reports additional corpus statistics, per-value and per-configuration results, ablation tables, and implementation details that complement the main text.

## S1. Moral value codes

To keep the result tables compact while preserving one column per value, we use short identifiers for each moral value. Table S1 lists the correspondence.

## S2. Direct DeBERTa

Tables S2 and S3 expand the direct DeBERTa results discussed in Section 6.3 of the main paper. They provide per-value validation and test $F_1$ scores for every configuration considered in Table 4 of the main paper, allowing

*Corresponding author
*Email address:* vicyesmo@upv.es (Víctor Yeste)

Table S1: Mapping between moral values and the short identifiers used in the suppelmentary material tables.

| **ID** | **Moral value** |
|---|---|
| V1 | Self-direction: thought |
| V2 | Self-direction: action |
| V3 | Stimulation |
| V4 | Hedonism |
| V5 | Achievement |
| V6 | Power: dominance |
| V7 | Power: resources |
| V8 | Face |
| V9 | Security: personal |
| V10 | Security: societal |
| V11 | Tradition |
| V12 | Conformity: rules |
| V13 | Conformity: interpersonal |
| V14 | Humility |
| V15 | Benevolence: caring |
| V16 | Benevolence: dependability |
| V17 | Universalism: concern |
| V18 | Universalism: nature |
| V19 | Universalism: tolerance |

a finer-grained inspection of which values benefit most from each auxiliary signal.

### *S2.1. Validation set*

Table S2 reports validation $F_1$-scores for all direct DeBERTa variants and all moral values (V1–V19), together with the macro-average.

### *S2.2. Test set*

## S3. Presence gate (DeBERTa)

Table S4 provides validation and test positive-class $F_1$ scores for all DeBERTa-based `presence` models. These results flesh out the summary in Table S4 and support the conclusions in Section 6.1 of the main paper about the narrow performance band around $F_1 \approx 0.73$–$0.74$. Table S4 lists all evaluated

presence-gate configurations, including their validation macro-$F_1$, test $F_1$ at $t = 0.5$, and test $F_1$ at the tuned threshold $t^\star$.

## S4. Hierarchical DeBERTa + presence gate

Tables S5 and S6–S7 detail the validation and test performance of all hierarchical configurations discussed in Section 6.2 of the main paper. They extend the comparison in Table 2 of the main paper by providing per-value $F_1$ scores and making explicit how different presence gates and decision thresholds affect the end-to-end macro-$F_1$.

### *S4.1. Validation set*

Table S5 shows validation $F_1$ for each moral value and the macro-average across all hierarchical pipelines.

### *S4.2. Test set*

Tables S6 and S7 report the corresponding test $F_1$ scores, including the thresholds for the value head and the presence gate.

## S5. Large Language Models

Tables S8 and S9 complement the summary in Table 5 of the main paper and the analysis in Section 6.4 of the main paper. They list per-configuration macro- and per-value $F_1$ scores for all LLM variants and ensembles, making it possible to trace the aggregate gains in Table 5 of the main paper back to individual models and prompts.

### *S5.1. Validation set*

Table S8 reports validation $F_1$ scores on each moral value and their macro-average for every LLM configuration (zero-shot, few-shot, and QLoRA).

### *S5.2. Test set*

Table S9 presents the corresponding test-set $F_1$ scores and underlies the best-single and best-ensemble LLM results discussed in Section 6.4 of the main paper.

## S6. Ensembles

This section expands the ensemble results summarised in Section S6 and discussed in Section 6.4 of the main paper. We list the individual members, voting scheme (hard, soft, or weighted), tuned thresholds, and full validation and test macro-$F_1$ scores for each ensemble configuration considered during forward selection. The goal is to make explicit how the final Transformer and LLM ensembles reported in Table 5 of the main paper were obtained and how much variance exists across closely related combinations.

### *S6.1. Transformer ensembles (by filter)*

Tables S10 and S11 detail the ensembles built from DeBERTa-based classifiers. Each row corresponds to one candidate ensemble considered in the forward-selection procedure of Section S6, with columns indicating the set of member models, the voting rule, the tuned global threshold $t^\star$, and the resulting macro-$F_1$ on the validation and test splits. These tables show that small, heterogeneous ensembles (mixing text-only and feature-augmented models) consistently outperform any single DeBERTa variant, underpinning the best supervised result ($F_1 = 0.332$) in Table 5 of the main paper.

### *S6.2. Transformer ensembles (presence)*

This subsection reports the full validation and test results for the Transformer-based ensembles used in the `presence` experiments. These ensembles combine the DeBERTa variants from Section 6.1 of the main paper via hard and soft voting under the same 8 GB GPU budget as the single models. We list, for each ensemble, its constituent runs, voting rule, and tuned decision thresholds so that the small differences between individual gates and ensembles can be inspected in detail. Unless stated otherwise, ensemble construction and selection follow the forward-selection procedure described in Section S6.

### *S6.3. Transformer ensembles (all)*

Here we summarise all Transformer-based ensembles considered, spanning presence-only gates, direct value detectors, and mixed configurations. The tables below expand the aggregate comparison in Table 5 of the main paper by providing validation and test macro-$F_1$ together with the exact component models and threshold choices for each ensemble. This detailed view complements the main-text discussion in Section 6.4 of the main paper and

allows readers to gauge how much each additional model contributes under the selection protocol of Section S6.

*S6.4. LLM ensembles*

Table S14 provides analogous details for the LLM-based ensembles. We include zero-shot, few-shot, and QLoRA-tuned Gemma-2-9B configurations, both with and without the SBERT presence gate, and report macro-$F_1$ for each ensemble candidate. These results complement the summary in Section 6.4 of the main paper: although individual LLM runs lag behind supervised DeBERTa, simple hard-voting ensembles of the strongest Gemma variants yield sizeable gains over their components and narrow (but do not close) the gap to the DeBERTa ensemble.

*S6.5. Hybrid ensembles*

This subsection explores mixed ensembles that combine DeBERTa-based classifiers with instruction-tuned LLMs. Table S15 reports the configuration of each mixed ensemble, together with its validation macro-$F_1$. In our setting, the best-performing mixed ensembles are competitive with purely Transformer-based ensembles but do not substantially improve over the compact soft-voting DeBERTa ensemble reported in Section 6.4 of the main paper.

## S7. Statistical tests

This section documents the full statistical tests underlying the significance statements in Section 4.9 of the main paper and throughout Section 6 of the main paper. We first summarise the main bootstrap comparisons on macro-$F_1$ between selected model pairs, then provide per-value McNemar analyses for those labels where differences remain significant after Benjamini–Hochberg FDR correction.

Tables S16 and S17 condense the bootstrap analysis described in Section 4.9 of the main paper for the key model pairs highlighted in Section 6 of the main paper. For each pair we report the test macro-$F_1$ of both systems, the point estimate of $\Delta$Macro-$F_1$ (improved minus reference), the one-sided lower 95% confidence bound, and the one-sided $p$-value for the hypothesis $\Delta > 0$. Comparisons where the lower bound is positive (and the $p$-value is small) correspond to claims of statistically reliable improvement in the main text; cases with overlapping intervals or large $p$-values are treated as inconclusive.

### *S7.1. Transformers*

This subsection lists the statistical comparisons for all Transformer-based systems discussed in Section 6 of the main paper. For each model pair we report test macro-$F_1$, the bootstrap estimate of $\Delta$Macro-$F_1$, the one-sided lower 95% confidence bound, and the corresponding one-sided $p$-value, following the protocol in Section 4.9 of the main paper.

### *S7.2. LLM*

This subsection mirrors the previous one for the instruction-tuned LLMs and their ensembles. We apply the same bootstrap procedure from Section 4.9 of the main paper to compare zero-shot, few-shot, QLoRA, and ensemble configurations, both within the LLM family and against the strongest Transformer baselines.

Table S2: Validation macro- and per-value F1-scores for all direct DeBERTa variants.

| Name | V1 | V2 | V3 | V4 | V5 | V6 | V7 | V8 | V9 | V10 | V11 | V12 | V13 | V14 | V15 | V16 | V17 | V18 | V19 | Macro-F1 |
|---|---|---|---|---|---|---|---|---|---|---|---|---|---|---|---|---|---|---|---|---|
| Baseline | 0.13 | 0.20 | 0.26 | 0.29 | 0.32 | 0.33 | 0.28 | 0.25 | 0.32 | 0.42 | 0.44 | 0.44 | 0.11 | 0.00 | 0.24 | 0.18 | 0.33 | 0.54 | 0.20 | 0.28 |
| Token Pruning (TP, IDF = 3.0) | 0.11 | 0.22 | 0.27 | 0.23 | 0.31 | 0.32 | 0.27 | 0.23 | 0.28 | 0.39 | 0.42 | 0.42 | 0.11 | 0.04 | 0.26 | 0.16 | 0.32 | 0.51 | 0.24 | 0.27 |
| 2 prev sentences with label | 0.10 | 0.24 | 0.30 | 0.30 | 0.37 | 0.33 | 0.29 | 0.27 | 0.35 | 0.44 | 0.45 | 0.45 | 0.09 | 0.00 | 0.19 | 0.22 | 0.35 | 0.57 | 0.22 | 0.29 |
| MultiLayer | 0.01 | 0.17 | 0.29 | 0.29 | 0.34 | 0.32 | 0.29 | 0.24 | 0.30 | 0.40 | 0.35 | 0.41 | 0.03 | 0.00 | 0.19 | 0.24 | 0.34 | 0.51 | 0.16 | 0.26 |
| Residual Block | 0.07 | 0.21 | 0.29 | 0.31 | 0.28 | 0.33 | 0.32 | 0.24 | 0.33 | 0.42 | 0.42 | 0.44 | 0.10 | 0.00 | 0.22 | 0.18 | 0.30 | 0.53 | 0.23 | 0.27 |
| Data Augmentation | 0.05 | 0.09 | 0.11 | 0.08 | 0.20 | 0.20 | 0.23 | 0.11 | 0.21 | 0.27 | 0.28 | 0.34 | 0.03 | 0.00 | 0.18 | 0.15 | 0.18 | 0.27 | 0.14 | 0.16 |
| Custom Stopwords | 0.12 | 0.20 | 0.26 | 0.33 | 0.31 | 0.30 | 0.34 | 0.23 | 0.32 | 0.41 | 0.44 | 0.45 | 0.10 | 0.00 | 0.23 | 0.21 | 0.31 | 0.56 | 0.19 | 0.28 |
| NER | 0.09 | 0.22 | 0.28 | 0.27 | 0.29 | 0.35 | 0.32 | 0.23 | 0.29 | 0.43 | 0.43 | 0.44 | 0.12 | 0.00 | 0.22 | 0.17 | 0.33 | 0.53 | 0.23 | 0.28 |
| Lex - Schwartz | 0.06 | 0.24 | 0.35 | 0.28 | 0.32 | 0.29 | 0.24 | 0.27 | 0.30 | 0.40 | 0.40 | 0.44 | 0.01 | 0.00 | 0.21 | 0.24 | 0.29 | 0.56 | 0.22 | 0.27 |
| Lex - VAD | 0.10 | 0.19 | 0.27 | 0.33 | 0.32 | 0.33 | 0.30 | 0.24 | 0.31 | 0.41 | 0.41 | 0.45 | 0.17 | 0.00 | 0.16 | 0.19 | 0.31 | 0.52 | 0.21 | 0.27 |
| Lex - EmoLex | 0.07 | 0.21 | 0.30 | 0.28 | 0.31 | 0.33 | 0.30 | 0.28 | 0.31 | 0.42 | 0.45 | 0.46 | 0.14 | 0.00 | 0.18 | 0.15 | 0.32 | 0.54 | 0.21 | 0.28 |
| Lex - Emotion Intensity | 0.10 | 0.24 | 0.29 | 0.35 | 0.28 | 0.35 | 0.31 | 0.25 | 0.31 | 0.42 | 0.40 | 0.44 | 0.17 | 0.00 | 0.20 | 0.18 | 0.32 | 0.54 | 0.17 | 0.28 |
| Lex - WorryWords | 0.08 | 0.24 | 0.32 | 0.30 | 0.33 | 0.32 | 0.26 | 0.25 | 0.28 | 0.40 | 0.43 | 0.42 | 0.01 | 0.00 | 0.22 | 0.22 | 0.28 | 0.57 | 0.17 | 0.27 |
| Lex - LIWC 15 | 0.10 | 0.19 | 0.26 | 0.28 | 0.32 | 0.33 | 0.28 | 0.23 | 0.31 | 0.40 | 0.41 | 0.45 | 0.09 | 0.00 | 0.26 | 0.24 | 0.33 | 0.52 | 0.25 | 0.28 |
| Lex - MFD | 0.05 | 0.25 | 0.34 | 0.27 | 0.32 | 0.30 | 0.26 | 0.28 | 0.30 | 0.40 | 0.39 | 0.44 | 0.01 | 0.00 | 0.21 | 0.23 | 0.29 | 0.56 | 0.23 | 0.27 |
| Lex - LIWC 22 | 0.13 | 0.23 | 0.31 | 0.30 | 0.30 | 0.36 | 0.27 | 0.26 | 0.34 | 0.43 | 0.44 | 0.44 | 0.18 | 0.00 | 0.19 | 0.22 | 0.30 | 0.54 | 0.23 | 0.29 |
| Lex - LIWC 22 + Linguistic Features | 0.07 | 0.20 | 0.31 | 0.27 | 0.32 | 0.36 | 0.30 | 0.25 | 0.33 | 0.43 | 0.42 | 0.45 | 0.17 | 0.00 | 0.22 | 0.21 | 0.35 | 0.54 | 0.19 | 0.28 |
| Lex - MFD-20 | 0.08 | 0.22 | 0.31 | 0.30 | 0.34 | 0.33 | 0.30 | 0.26 | 0.32 | 0.42 | 0.42 | 0.42 | 0.02 | 0.00 | 0.24 | 0.24 | 0.26 | 0.57 | 0.19 | 0.28 |
| Lex - eMFD | 0.08 | 0.22 | 0.30 | 0.27 | 0.35 | 0.32 | 0.30 | 0.25 | 0.34 | 0.42 | 0.41 | 0.43 | 0.00 | 0.00 | 0.25 | 0.26 | 0.26 | 0.57 | 0.21 | 0.28 |
| Lex - MJD | 0.06 | 0.23 | 0.32 | 0.29 | 0.35 | 0.34 | 0.27 | 0.27 | 0.33 | 0.41 | 0.42 | 0.44 | 0.00 | 0.00 | 0.21 | 0.27 | 0.27 | 0.58 | 0.22 | 0.28 |
| Topic Detection - LDA | 0.09 | 0.23 | 0.27 | 0.35 | 0.31 | 0.35 | 0.30 | 0.20 | 0.31 | 0.43 | 0.45 | 0.45 | 0.16 | 0.00 | 0.17 | 0.19 | 0.31 | 0.50 | 0.22 | 0.28 |
| Topic Detection - NMF | 0.10 | 0.22 | 0.29 | 0.33 | 0.31 | 0.36 | 0.29 | 0.25 | 0.31 | 0.43 | 0.44 | 0.44 | 0.11 | 0.00 | 0.20 | 0.18 | 0.30 | 0.56 | 0.24 | 0.28 |
| Topic Detection - BERTopic | 0.08 | 0.22 | 0.29 | 0.34 | 0.31 | 0.35 | 0.31 | 0.24 | 0.33 | 0.42 | 0.44 | 0.43 | 0.16 | 0.00 | 0.21 | 0.21 | 0.33 | 0.54 | 0.21 | 0.29 |

Table S3: Test macro- and per-value F1-scores for all direct DeBERTa variants.

| **Name** | **Thr** | **V1** | **V2** | **V3** | **V4** | **V5** | **V6** | **V7** | **V8** | **V9** | **V10** | **V11** | **V12** | **V13** | **V14** | **V15** | **V16** | **V17** | **V18** | **V19** | **Macro-F1** |
|---|---|---|---|---|---|---|---|---|---|---|---|---|---|---|---|---|---|---|---|---|---|
| Baseline | 0.5 | 0.12 | 0.19 | 0.28 | 0.31 | 0.34 | 0.32 | 0.33 | 0.17 | 0.35 | 0.41 | 0.47 | 0.43 | 0.11 | 0 | 0.2 | 0.19 | 0.37 | 0.57 | 0.19 | 0.28112 |
| 2 prev sentences with label | 0.5 | 0.07 | 0.19 | 0.26 | 0.33 | 0.35 | 0.31 | 0.35 | 0.19 | 0.38 | 0.4 | 0.46 | 0.43 | 0.08 | 0 | 0.19 | 0.2 | 0.42 | 0.58 | 0.19 | 0.28181 |
| Lex - LIWC 22 | 0.5 | 0.16 | 0.21 | 0.26 | 0.3 | 0.32 | 0.33 | 0.35 | 0.23 | 0.32 | 0.41 | 0.49 | 0.44 | 0.1 | 0 | 0.16 | 0.23 | 0.37 | 0.54 | 0.22 | 0.28593 |
| Topic Detection - BERTopic | 0.5 | 0.14 | 0.21 | 0.27 | 0.31 | 0.31 | 0.34 | 0.36 | 0.2 | 0.33 | 0.42 | 0.47 | 0.42 | 0.09 | 0 | 0.17 | 0.2 | 0.38 | 0.56 | 0.22 | 0.28413 |
| Baseline | 0.3 | 0.16 | 0.21 | 0.3 | 0.29 | 0.38 | 0.33 | 0.39 | 0.21 | 0.34 | 0.43 | 0.46 | 0.43 | 0.17 | 0.06 | 0.24 | 0.28 | 0.43 | 0.58 | 0.23 | 0.31149 |
| 2 prev sentences with label | 0.15 | 0.14 | 0.24 | 0.29 | 0.33 | 0.37 | 0.35 | 0.4 | 0.24 | 0.37 | 0.43 | 0.45 | 0.43 | 0.14 | 0.05 | 0.27 | 0.31 | 0.41 | 0.55 | 0.26 | 0.31771 |
| Lex - LIWC 22 | 0.25 | 0.19 | 0.22 | 0.29 | 0.28 | 0.37 | 0.35 | 0.41 | 0.26 | 0.35 | 0.42 | 0.47 | 0.46 | 0.17 | 0.06 | 0.26 | 0.31 | 0.42 | 0.56 | 0.24 | 0.31986 |
| Topic Detection - BERTopic | 0.2 | 0.19 | 0.22 | 0.28 | 0.31 | 0.37 | 0.34 | 0.4 | 0.26 | 0.37 | 0.42 | 0.47 | 0.44 | 0.15 | 0 | 0.27 | 0.3 | 0.42 | 0.55 | 0.28 | 0.31871 |

Statistical tests

Table S4: Presence gate variants based on DeBERTa: validation and test macro-average F1-scores. Test scoring was applied only to baseline and best variants.

| Name | Val Macro-F1 | Test Macro-F1 (0.5) | Best thr | Test Macro-F1 (tuned) |
|---|---|---|---|---|
| Baseline | 0.62 | 0.74 | 0.1 | 0.73 |
| Token Pruning (TP, IDF = 3.0) | 0.63 | | | |
| 2 prev sentences with label | 0.65 | | | |
| MultiLayer | 0.62 | | | |
| Residual Block | 0.62 | | | |
| Data Augmentation | 0.61 | | | |
| Custom Stopwords | 0.61 | | | |
| NER | 0.62 | | | |
| Lex - Schwartz | 0.62 | | | |
| Lex - VAD | 0.61 | | | |
| Lex - EmoLex | 0.64 | | | |
| Lex - Emotion Intensity | 0.62 | | | |
| Lex - WorryWords | 0.64 | | | |
| Lex - LIWC 15 | 0.62 | | | |
| Lex - MFD | 0.63 | | | |
| Lex - LIWC 22 | 0.63 | | | |
| Lex - LIWC 22 + Linguistic Features | 0.74 | 0.74 | 0.1 | 0.74 |
| Lex - MFD-20 | 0.62 | | | |
| Lex - eMFD | 0.66 | | | |
| Lex - MJD | 0.62 | | | |
| Topic Detection - LDA | 0.61 | | | |
| Topic Detection - NMF | 0.61 | | | |
| Topic Detection - BERTopic | 0.62 | | | |
| 2 prev sentences with label + Token Pruning (TP, IDF = 3.0) | 0.65 | | | |
| 2 prev sentences with label + EmoLex | 0.67 | 0.73 | 0.1 | 0.74 |
| 2 prev sentences with label + WorryWords | 0.66 | | | |
| 2 prev sentences with label + MFD | 0.66 | | | |
| 2 prev sentences with label + LIWC 22 | 0.67 | 0.73 | 0.1 | 0.74 |
| 2 prev sentences with label + eMFD | 0.67 | 0.73 | 0.1 | 0.74 |

Table S5: Hierarchical DeBERTa with presence gate: validation F1-scores per moral value (V1–V19) and macro-average (Macro-F1).

| Name | V1 | V2 | V3 | V4 | V5 | V6 | V7 | V8 | V9 | V10 | V11 | V12 | V13 | V14 | V15 | V16 | V17 | V18 | V19 | Macro-F1 |
|---|---|---|---|---|---|---|---|---|---|---|---|---|---|---|---|---|---|---|---|---|
| Baseline | 0.19 | 0.29 | 0.39 | 0.38 | 0.48 | 0.44 | 0.45 | 0.34 | 0.47 | 0.51 | 0.51 | 0.59 | 0.14 | 0 | 0.28 | 0.3 | 0.4 | 0.67 | 0.26 | 0.37 |
| Token Pruning (TP, IDF = 3.0) | 0.16 | 0.3 | 0.39 | 0.4 | 0.47 | 0.42 | 0.45 | 0.27 | 0.44 | 0.52 | 0.51 | 0.56 | 0.2 | 0 | 0.28 | 0.27 | 0.36 | 0.67 | 0.28 | 0.37 |
| 2 prev sentences with label | 0.15 | 0.3 | 0.39 | 0.44 | 0.48 | 0.42 | 0.46 | 0.31 | 0.45 | 0.52 | 0.52 | 0.56 | 0.14 | 0 | 0.23 | 0.3 | 0.41 | 0.65 | 0.29 | 0.37 |
| MultiLayer | 0.01 | 0.24 | 0.36 | 0.41 | 0.47 | 0.4 | 0.43 | 0.32 | 0.42 | 0.51 | 0.54 | 0.55 | 0.08 | 0 | 0.26 | 0.3 | 0.38 | 0.65 | 0.26 | 0.35 |
| Residual Block | 0.1 | 0.29 | 0.35 | 0.41 | 0.49 | 0.43 | 0.42 | 0.33 | 0.48 | 0.53 | 0.51 | 0.6 | 0.14 | 0 | 0.31 | 0.31 | 0.4 | 0.66 | 0.3 | 0.38 |
| Data Augmentation | 0.11 | 0.2 | 0.2 | 0.24 | 0.36 | 0.32 | 0.33 | 0.19 | 0.39 | 0.43 | 0.34 | 0.4 | 0 | 0 | 0.21 | 0.16 | 0.26 | 0.54 | 0.18 | 0.26 |
| Custom Stopwords | 0.16 | 0.28 | 0.37 | 0.35 | 0.47 | 0.38 | 0.42 | 0.32 | 0.44 | 0.52 | 0.53 | 0.58 | 0.17 | 0 | 0.28 | 0.28 | 0.41 | 0.68 | 0.31 | 0.37 |
| NER | 0.17 | 0.31 | 0.36 | 0.39 | 0.49 | 0.42 | 0.43 | 0.3 | 0.46 | 0.52 | 0.51 | 0.58 | 0.17 | 0 | 0.28 | 0.32 | 0.36 | 0.67 | 0.3 | 0.37 |
| Lex - Schwartz | 0.17 | 0.31 | 0.36 | 0.41 | 0.48 | 0.39 | 0.45 | 0.32 | 0.46 | 0.5 | 0.5 | 0.55 | 0.15 | 0 | 0.29 | 0.3 | 0.38 | 0.67 | 0.26 | 0.37 |
| Lex - VAD | 0.18 | 0.29 | 0.37 | 0.37 | 0.47 | 0.41 | 0.41 | 0.33 | 0.45 | 0.51 | 0.5 | 0.57 | 0.18 | 0 | 0.3 | 0.31 | 0.39 | 0.68 | 0.27 | 0.37 |
| Lex - EmoLex | 0.19 | 0.3 | 0.37 | 0.4 | 0.5 | 0.42 | 0.42 | 0.32 | 0.42 | 0.53 | 0.53 | 0.6 | 0.2 | 0 | 0.3 | 0.3 | 0.39 | 0.67 | 0.26 | 0.37 |
| Lex - Emotion Intensity | 0.17 | 0.31 | 0.35 | 0.44 | 0.48 | 0.42 | 0.45 | 0.31 | 0.46 | 0.52 | 0.54 | 0.56 | 0.18 | 0.04 | 0.27 | 0.31 | 0.38 | 0.68 | 0.29 | 0.38 |
| Lex - WorryWords | 0.16 | 0.3 | 0.35 | 0.43 | 0.5 | 0.44 | 0.39 | 0.33 | 0.45 | 0.51 | 0.52 | 0.58 | 0.16 | 0 | 0.33 | 0.31 | 0.39 | 0.66 | 0.27 | 0.37 |
| Lex - LIWC 15 | 0.19 | 0.3 | 0.38 | 0.42 | 0.48 | 0.42 | 0.48 | 0.31 | 0.46 | 0.51 | 0.51 | 0.55 | 0.17 | 0 | 0.29 | 0.3 | 0.41 | 0.68 | 0.27 | 0.38 |
| Lex - MFD | 0.14 | 0.24 | 0.34 | 0.42 | 0.5 | 0.39 | 0.47 | 0.31 | 0.44 | 0.51 | 0.49 | 0.57 | 0.14 | 0 | 0.31 | 0.3 | 0.35 | 0.66 | 0.21 | 0.36 |
| Lex - LIWC 22 | 0.19 | 0.32 | 0.37 | 0.41 | 0.49 | 0.45 | 0.42 | 0.3 | 0.46 | 0.5 | 0.52 | 0.59 | 0.15 | 0 | 0.28 | 0.34 | 0.4 | 0.67 | 0.29 | 0.38 |
| Lex - LIWC 22 + Linguistic Features | 0.16 | 0.31 | 0.35 | 0.4 | 0.5 | 0.42 | 0.42 | 0.32 | 0.46 | 0.53 | 0.52 | 0.57 | 0.16 | 0 | 0.31 | 0.32 | 0.41 | 0.67 | 0.3 | 0.38 |
| Lex - MFD-20 | 0.11 | 0.3 | 0.35 | 0.43 | 0.5 | 0.38 | 0.42 | 0.31 | 0.44 | 0.54 | 0.52 | 0.57 | 0.22 | 0 | 0.32 | 0.33 | 0.38 | 0.68 | 0.33 | 0.38 |
| Lex - eMFD | 0.11 | 0.3 | 0.35 | 0.44 | 0.5 | 0.37 | 0.42 | 0.32 | 0.46 | 0.54 | 0.52 | 0.57 | 0.2 | 0 | 0.33 | 0.33 | 0.38 | 0.67 | 0.33 | 0.38 |
| Lex - MJD | 0.19 | 0.33 | 0.39 | 0.42 | 0.49 | 0.44 | 0.45 | 0.33 | 0.45 | 0.51 | 0.52 | 0.59 | 0.18 | 0 | 0.29 | 0.28 | 0.36 | 0.65 | 0.28 | 0.38 |
| Topic Detection - LDA | 0.17 | 0.3 | 0.39 | 0.36 | 0.49 | 0.42 | 0.42 | 0.33 | 0.44 | 0.51 | 0.51 | 0.6 | 0.16 | 0 | 0.34 | 0.28 | 0.37 | 0.68 | 0.29 | 0.37 |
| Topic Detection - NMF | 0.17 | 0.3 | 0.39 | 0.38 | 0.48 | 0.43 | 0.42 | 0.34 | 0.44 | 0.51 | 0.51 | 0.6 | 0.16 | 0 | 0.32 | 0.28 | 0.37 | 0.68 | 0.29 | 0.37 |
| Topic Detection - BERTopic | 0.19 | 0.31 | 0.39 | 0.36 | 0.49 | 0.43 | 0.41 | 0.32 | 0.45 | 0.51 | 0.51 | 0.6 | 0.15 | 0 | 0.33 | 0.3 | 0.37 | 0.67 | 0.3 | 0.37 |
| 2 prev sentences with label + Residual Block | 0.21 | 0.33 | 0.34 | 0.41 | 0.49 | 0.42 | 0.46 | 0.33 | 0.46 | 0.52 | 0.52 | 0.55 | 0.21 | 0.04 | 0.25 | 0.31 | 0.4 | 0.67 | 0.26 | 0.38 |
| 2 prev sentences with label + VAD | 0.19 | 0.28 | 0.37 | 0.42 | 0.49 | 0.42 | 0.44 | 0.29 | 0.46 | 0.5 | 0.55 | 0.56 | 0.23 | 0.04 | 0.27 | 0.29 | 0.39 | 0.68 | 0.27 | 0.38 |
| 2 prev sentences with label + EmoLex | 0.19 | 0.29 | 0.36 | 0.42 | 0.44 | 0.42 | 0.43 | 0.33 | 0.45 | 0.54 | 0.5 | 0.56 | 0.2 | 0 | 0.27 | 0.28 | 0.37 | 0.67 | 0.27 | 0.37 |
| 2 prev sentences with label + Emotion Intensity | 0.16 | 0.3 | 0.4 | 0.39 | 0.46 | 0.42 | 0.45 | 0.31 | 0.48 | 0.53 | 0.52 | 0.55 | 0.21 | 0 | 0.29 | 0.23 | 0.37 | 0.64 | 0.27 | 0.37 |
| 2 prev sentences with label + WorryWords | 0.15 | 0.29 | 0.37 | 0.4 | 0.49 | 0.4 | 0.43 | 0.32 | 0.49 | 0.52 | 0.51 | 0.54 | 0.16 | 0.04 | 0.21 | 0.31 | 0.4 | 0.65 | 0.28 | 0.37 |
| 2 prev sentences with label + LIWC 15 | 0.14 | 0.28 | 0.41 | 0.41 | 0.46 | 0.42 | 0.45 | 0.28 | 0.48 | 0.53 | 0.51 | 0.57 | 0.18 | 0 | 0.29 | 0.25 | 0.38 | 0.66 | 0.25 | 0.37 |
| 2 prev sentences with label + LIWC 22 | 0.18 | 0.29 | 0.39 | 0.42 | 0.47 | 0.39 | 0.45 | 0.31 | 0.47 | 0.54 | 0.54 | 0.58 | 0.24 | 0.04 | 0.33 | 0.3 | 0.38 | 0.66 | 0.3 | 0.38 |
| 2 prev sentences with label + MFD-20 | 0.21 | 0.3 | 0.38 | 0.46 | 0.5 | 0.39 | 0.46 | 0.32 | 0.45 | 0.52 | 0.51 | 0.56 | 0.19 | 0 | 0.24 | 0.27 | 0.42 | 0.66 | 0.3 | 0.38 |
| 2 prev sentences with label + eMFD | 0.14 | 0.27 | 0.39 | 0.47 | 0.46 | 0.41 | 0.47 | 0.34 | 0.48 | 0.52 | 0.53 | 0.55 | 0.21 | 0.04 | 0.29 | 0.26 | 0.41 | 0.66 | 0.28 | 0.38 |
| 2 prev sentences with label + MJD | 0.2 | 0.29 | 0.39 | 0.39 | 0.48 | 0.43 | 0.46 | 0.32 | 0.47 | 0.53 | 0.53 | 0.57 | 0.2 | 0.04 | 0.29 | 0.28 | 0.39 | 0.68 | 0.27 | 0.38 |
| Residual Block + VAD | 0.16 | 0.31 | 0.37 | 0.46 | 0.5 | 0.38 | 0.44 | 0.33 | 0.47 | 0.54 | 0.52 | 0.56 | 0.18 | 0 | 0.29 | 0.33 | 0.41 | 0.67 | 0.27 | 0.38 |
| Residual Block + EmoLex | 0.15 | 0.32 | 0.38 | 0.4 | 0.49 | 0.41 | 0.45 | 0.33 | 0.45 | 0.53 | 0.53 | 0.57 | 0.21 | 0 | 0.29 | 0.3 | 0.4 | 0.68 | 0.3 | 0.38 |
| Residual Block + Emotion Intensity | 0.12 | 0.31 | 0.38 | 0.45 | 0.48 | 0.42 | 0.48 | 0.32 | 0.46 | 0.52 | 0.54 | 0.56 | 0.21 | 0 | 0.27 | 0.31 | 0.38 | 0.67 | 0.26 | 0.38 |
| Residual Block + WorryWords | 0.18 | 0.3 | 0.36 | 0.43 | 0.49 | 0.44 | 0.47 | 0.31 | 0.45 | 0.51 | 0.51 | 0.6 | 0.15 | 0 | 0.3 | 0.3 | 0.37 | 0.67 | 0.29 | 0.38 |
| Residual Block + LIWC 15 | 0.17 | 0.3 | 0.38 | 0.36 | 0.49 | 0.44 | 0.45 | 0.31 | 0.47 | 0.51 | 0.53 | 0.58 | 0.16 | 0 | 0.33 | 0.33 | 0.38 | 0.66 | 0.28 | 0.38 |
| Residual Block + LIWC 22 | 0.21 | 0.33 | 0.37 | 0.39 | 0.49 | 0.43 | 0.42 | 0.32 | 0.45 | 0.51 | 0.52 | 0.58 | 0.21 | 0 | 0.32 | 0.35 | 0.37 | 0.67 | 0.31 | 0.38 |
| Residual Block + MFD-20 | 0.16 | 0.29 | 0.37 | 0.45 | 0.49 | 0.39 | 0.44 | 0.33 | 0.43 | 0.55 | 0.49 | 0.57 | 0.21 | 0.04 | 0.27 | 0.32 | 0.41 | 0.68 | 0.28 | 0.38 |
| Residual Block + eMFD | 0.14 | 0.3 | 0.35 | 0.44 | 0.5 | 0.38 | 0.44 | 0.32 | 0.43 | 0.54 | 0.49 | 0.57 | 0.2 | 0.04 | 0.3 | 0.32 | 0.41 | 0.67 | 0.29 | 0.38 |
| Residual Block + MJD | 0.17 | 0.31 | 0.37 | 0.4 | 0.5 | 0.42 | 0.46 | 0.31 | 0.44 | 0.52 | 0.53 | 0.57 | 0.19 | 0 | 0.3 | 0.29 | 0.41 | 0.67 | 0.27 | 0.38 |

Table S6: Hierarchical DeBERTa with presence gate: test F1-scores per moral value (V1–V19), for different thresholds and filter models, and macro-average (Macro-F1). Part 1.

| Name | Thr | Filter | Filter thr | V1 | V2 | V3 | V4 | V5 | V6 | V7 | V8 | V9 | V10 | V11 | V12 | V13 | V14 | V15 | V16 | V17 | V18 | V19 | Macro-F1 |
|---|---|---|---|---|---|---|---|---|---|---|---|---|---|---|---|---|---|---|---|---|---|---|---|
| Baseline | 0.5 | Baseline | 0.5 | 0.11 | 0.2 | 0.26 | 0.3 | 0.33 | 0.32 | 0.36 | 0.2 | 0.35 | 0.4 | 0.45 | 0.44 | 0.07 | 0 | 0.23 | 0.25 | 0.39 | 0.56 | 0.2 | 0.284 |
| Baseline | 0.5 | Lex-LIWC-22_LingFeat | 0.5 | 0.12 | 0.19 | 0.27 | 0.3 | 0.34 | 0.32 | 0.35 | 0.22 | 0.35 | 0.4 | 0.48 | 0.43 | 0.06 | 0 | 0.22 | 0.27 | 0.38 | 0.57 | 0.2 | 0.288 |
| Baseline | 0.5 | Lex-LIWC-22_LingFeat | 0.1 | 0.12 | 0.2 | 0.27 | 0.33 | 0.34 | 0.32 | 0.36 | 0.23 | 0.34 | 0.39 | 0.47 | 0.43 | 0.07 | 0 | 0.24 | 0.27 | 0.39 | 0.56 | 0.22 | 0.293 |
| Baseline | 0.5 | Previous-Sentences-2-Lex-EmoLex | 0.1 | 0.11 | 0.2 | 0.27 | 0.3 | 0.34 | 0.33 | 0.36 | 0.23 | 0.35 | 0.39 | 0.47 | 0.42 | 0.07 | 0 | 0.24 | 0.27 | 0.4 | 0.56 | 0.22 | 0.29 |
| Baseline | 0.5 | Previous-Sentences-2-Lex-LIWC-22 | 0.1 | 0.12 | 0.2 | 0.27 | 0.33 | 0.34 | 0.33 | 0.36 | 0.24 | 0.34 | 0.39 | 0.47 | 0.42 | 0.06 | 0 | 0.23 | 0.27 | 0.4 | 0.55 | 0.22 | 0.293 |
| Baseline | 0.5 | Previous-Sentences-2-Lex-eMFD | 0.1 | 0.09 | 0.2 | 0.29 | 0.29 | 0.34 | 0.33 | 0.35 | 0.23 | 0.34 | 0.39 | 0.46 | 0.42 | 0.06 | 0 | 0.23 | 0.28 | 0.4 | 0.55 | 0.2 | 0.286 |
| 2 prev sentences with label | 0.5 | Baseline | 0.5 | 0.11 | 0.2 | 0.24 | 0.3 | 0.33 | 0.3 | 0.39 | 0.18 | 0.33 | 0.41 | 0.42 | 0.45 | 0.07 | 0 | 0.23 | 0.24 | 0.39 | 0.57 | 0.27 | 0.285 |
| 2 prev sentences with label | 0.5 | Lex-LIWC-22_LingFeat | 0.5 | 0.11 | 0.19 | 0.28 | 0.3 | 0.34 | 0.31 | 0.37 | 0.2 | 0.35 | 0.4 | 0.46 | 0.44 | 0.06 | 0 | 0.21 | 0.25 | 0.4 | 0.57 | 0.27 | 0.289 |
| 2 prev sentences with label | 0.5 | Lex-LIWC-22_LingFeat | 0.1 | 0.11 | 0.2 | 0.26 | 0.33 | 0.33 | 0.32 | 0.37 | 0.22 | 0.34 | 0.4 | 0.43 | 0.44 | 0.07 | 0 | 0.24 | 0.25 | 0.4 | 0.58 | 0.27 | 0.292 |
| 2 prev sentences with label | 0.5 | Previous-Sentences-2-Lex-EmoLex | 0.1 | 0.09 | 0.19 | 0.26 | 0.3 | 0.34 | 0.32 | 0.37 | 0.22 | 0.35 | 0.4 | 0.44 | 0.43 | 0.07 | 0 | 0.24 | 0.26 | 0.4 | 0.56 | 0.27 | 0.29 |
| 2 prev sentences with label | 0.5 | Previous-Sentences-2-Lex-LIWC-22 | 0.1 | 0.12 | 0.2 | 0.24 | 0.31 | 0.34 | 0.33 | 0.37 | 0.23 | 0.34 | 0.39 | 0.43 | 0.43 | 0.07 | 0 | 0.24 | 0.26 | 0.4 | 0.57 | 0.26 | 0.292 |
| 2 prev sentences with label | 0.5 | Previous-Sentences-2-Lex-eMFD | 0.1 | 0.09 | 0.2 | 0.27 | 0.32 | 0.33 | 0.33 | 0.36 | 0.22 | 0.34 | 0.4 | 0.44 | 0.43 | 0.07 | 0 | 0.24 | 0.26 | 0.4 | 0.57 | 0.26 | 0.291 |
| Residual Block | 0.5 | Baseline | 0.5 | 0.06 | 0.2 | 0.27 | 0.31 | 0.35 | 0.32 | 0.34 | 0.19 | 0.34 | 0.4 | 0.47 | 0.43 | 0.08 | 0 | 0.24 | 0.25 | 0.38 | 0.57 | 0.23 | 0.285 |
| Residual Block | 0.5 | Lex-LIWC-22_LingFeat | 0.5 | 0.07 | 0.19 | 0.28 | 0.29 | 0.35 | 0.31 | 0.33 | 0.19 | 0.35 | 0.4 | 0.49 | 0.43 | 0.07 | 0 | 0.23 | 0.26 | 0.38 | 0.58 | 0.23 | 0.286 |
| Residual Block | 0.5 | Lex-LIWC-22_LingFeat | 0.1 | 0.08 | 0.21 | 0.27 | 0.32 | 0.35 | 0.32 | 0.34 | 0.2 | 0.35 | 0.4 | 0.48 | 0.43 | 0.08 | 0 | 0.25 | 0.27 | 0.38 | 0.57 | 0.25 | 0.292 |
| Residual Block | 0.5 | Previous-Sentences-2-Lex-EmoLex | 0.1 | 0.06 | 0.2 | 0.28 | 0.29 | 0.35 | 0.33 | 0.34 | 0.22 | 0.35 | 0.4 | 0.48 | 0.42 | 0.08 | 0 | 0.24 | 0.27 | 0.39 | 0.57 | 0.25 | 0.29 |
| Residual Block | 0.5 | Previous-Sentences-2-Lex-LIWC-22 | 0.1 | 0.09 | 0.2 | 0.28 | 0.32 | 0.35 | 0.32 | 0.35 | 0.22 | 0.35 | 0.4 | 0.48 | 0.43 | 0.07 | 0 | 0.24 | 0.27 | 0.38 | 0.57 | 0.24 | 0.292 |
| Residual Block | 0.5 | Previous-Sentences-2-Lex-eMFD | 0.1 | 0.05 | 0.2 | 0.28 | 0.3 | 0.34 | 0.32 | 0.33 | 0.2 | 0.34 | 0.39 | 0.47 | 0.43 | 0.07 | 0 | 0.25 | 0.27 | 0.39 | 0.57 | 0.24 | 0.287 |
| Lex - VAD | 0.5 | Baseline | 0.5 | 0.13 | 0.19 | 0.26 | 0.26 | 0.34 | 0.32 | 0.35 | 0.19 | 0.34 | 0.41 | 0.45 | 0.45 | 0.11 | 0 | 0.23 | 0.29 | 0.4 | 0.59 | 0.23 | 0.292 |
| Lex - VAD | 0.5 | Lex-LIWC-22_LingFeat | 0.5 | 0.12 | 0.19 | 0.26 | 0.26 | 0.35 | 0.32 | 0.34 | 0.19 | 0.35 | 0.42 | 0.48 | 0.44 | 0.1 | 0 | 0.22 | 0.29 | 0.4 | 0.6 | 0.23 | 0.293 |
| Lex - VAD | 0.5 | Lex-LIWC-22_LingFeat | 0.1 | 0.13 | 0.2 | 0.26 | 0.28 | 0.35 | 0.32 | 0.35 | 0.22 | 0.35 | 0.41 | 0.46 | 0.44 | 0.11 | 0 | 0.24 | 0.3 | 0.4 | 0.58 | 0.24 | 0.297 |
| Lex - VAD | 0.5 | Previous-Sentences-2-Lex-EmoLex | 0.1 | 0.12 | 0.19 | 0.26 | 0.25 | 0.36 | 0.33 | 0.35 | 0.22 | 0.35 | 0.41 | 0.47 | 0.43 | 0.12 | 0 | 0.24 | 0.3 | 0.41 | 0.59 | 0.25 | 0.297 |
| Lex - VAD | 0.5 | Previous-Sentences-2-Lex-LIWC-22 | 0.1 | 0.13 | 0.19 | 0.26 | 0.28 | 0.35 | 0.32 | 0.35 | 0.23 | 0.34 | 0.41 | 0.46 | 0.44 | 0.1 | 0 | 0.24 | 0.3 | 0.41 | 0.58 | 0.25 | 0.297 |
| Lex - VAD | 0.5 | Previous-Sentences-2-Lex-eMFD | 0.1 | 0.11 | 0.19 | 0.26 | 0.24 | 0.35 | 0.33 | 0.34 | 0.22 | 0.35 | 0.41 | 0.46 | 0.44 | 0.1 | 0 | 0.24 | 0.3 | 0.41 | 0.58 | 0.24 | 0.294 |
| Lex - EmoLex | 0.5 | Baseline | 0.5 | 0.08 | 0.18 | 0.26 | 0.27 | 0.35 | 0.32 | 0.33 | 0.22 | 0.33 | 0.41 | 0.44 | 0.44 | 0.08 | 0 | 0.23 | 0.26 | 0.39 | 0.58 | 0.26 | 0.286 |
| Lex - EmoLex | 0.5 | Lex-LIWC-22_LingFeat | 0.5 | 0.07 | 0.18 | 0.28 | 0.26 | 0.36 | 0.32 | 0.32 | 0.22 | 0.33 | 0.41 | 0.46 | 0.44 | 0.07 | 0 | 0.22 | 0.27 | 0.39 | 0.59 | 0.27 | 0.288 |
| Lex - EmoLex | 0.5 | Lex-LIWC-22_LingFeat | 0.1 | 0.09 | 0.2 | 0.27 | 0.3 | 0.36 | 0.32 | 0.33 | 0.24 | 0.33 | 0.4 | 0.45 | 0.44 | 0.08 | 0 | 0.25 | 0.27 | 0.39 | 0.57 | 0.28 | 0.293 |
| Lex - EmoLex | 0.5 | Previous-Sentences-2-Lex-EmoLex | 0.1 | 0.08 | 0.19 | 0.27 | 0.26 | 0.36 | 0.32 | 0.33 | 0.24 | 0.33 | 0.4 | 0.46 | 0.43 | 0.07 | 0 | 0.24 | 0.27 | 0.4 | 0.57 | 0.28 | 0.291 |
| Lex - EmoLex | 0.5 | Previous-Sentences-2-Lex-LIWC-22 | 0.1 | 0.1 | 0.2 | 0.26 | 0.3 | 0.36 | 0.32 | 0.34 | 0.26 | 0.32 | 0.4 | 0.45 | 0.44 | 0.07 | 0 | 0.24 | 0.27 | 0.4 | 0.58 | 0.27 | 0.294 |
| Lex - EmoLex | 0.5 | Previous-Sentences-2-Lex-eMFD | 0.1 | 0.07 | 0.19 | 0.27 | 0.27 | 0.35 | 0.33 | 0.33 | 0.25 | 0.33 | 0.4 | 0.46 | 0.44 | 0.08 | 0 | 0.24 | 0.28 | 0.4 | 0.58 | 0.27 | 0.29 |
| Lex - Emotion Intensity | 0.5 | Baseline | 0.5 | 0.08 | 0.21 | 0.25 | 0.26 | 0.33 | 0.31 | 0.36 | 0.21 | 0.33 | 0.41 | 0.49 | 0.44 | 0.13 | 0 | 0.2 | 0.28 | 0.38 | 0.56 | 0.24 | 0.288 |
| Lex - Emotion Intensity | 0.5 | Lex-LIWC-22_LingFeat | 0.5 | 0.08 | 0.21 | 0.27 | 0.27 | 0.34 | 0.32 | 0.36 | 0.21 | 0.33 | 0.42 | 0.5 | 0.43 | 0.13 | 0 | 0.19 | 0.28 | 0.38 | 0.57 | 0.23 | 0.29 |
| Lex - Emotion Intensity | 0.5 | Lex-LIWC-22_LingFeat | 0.1 | 0.08 | 0.22 | 0.26 | 0.27 | 0.34 | 0.31 | 0.35 | 0.22 | 0.33 | 0.4 | 0.48 | 0.43 | 0.12 | 0 | 0.22 | 0.28 | 0.38 | 0.55 | 0.25 | 0.29 |
| Lex - Emotion Intensity | 0.5 | Previous-Sentences-2-Lex-EmoLex | 0.1 | 0.08 | 0.21 | 0.27 | 0.24 | 0.34 | 0.32 | 0.35 | 0.23 | 0.33 | 0.4 | 0.48 | 0.43 | 0.12 | 0 | 0.22 | 0.28 | 0.38 | 0.56 | 0.25 | 0.289 |
| Lex - Emotion Intensity | 0.5 | Previous-Sentences-2-Lex-LIWC-22 | 0.1 | 0.1 | 0.21 | 0.26 | 0.28 | 0.34 | 0.32 | 0.36 | 0.23 | 0.33 | 0.4 | 0.48 | 0.43 | 0.12 | 0 | 0.21 | 0.28 | 0.38 | 0.55 | 0.25 | 0.291 |
| Lex - Emotion Intensity | 0.5 | Previous-Sentences-2-Lex-eMFD | 0.1 | 0.07 | 0.22 | 0.27 | 0.25 | 0.33 | 0.32 | 0.34 | 0.22 | 0.33 | 0.4 | 0.48 | 0.43 | 0.13 | 0 | 0.22 | 0.29 | 0.38 | 0.55 | 0.25 | 0.288 |
| Lex - WorryWords | 0.5 | Baseline | 0.5 | 0.1 | 0.19 | 0.24 | 0.28 | 0.35 | 0.32 | 0.33 | 0.2 | 0.34 | 0.4 | 0.45 | 0.45 | 0.08 | 0 | 0.26 | 0.29 | 0.38 | 0.57 | 0.26 | 0.289 |
| Lex - WorryWords | 0.5 | Lex-LIWC-22_LingFeat | 0.5 | 0.11 | 0.18 | 0.25 | 0.28 | 0.36 | 0.32 | 0.32 | 0.21 | 0.34 | 0.41 | 0.48 | 0.44 | 0.07 | 0 | 0.25 | 0.3 | 0.38 | 0.58 | 0.24 | 0.291 |
| Lex - WorryWords | 0.5 | Lex-LIWC-22_LingFeat | 0.1 | 0.1 | 0.2 | 0.26 | 0.32 | 0.36 | 0.32 | 0.34 | 0.23 | 0.34 | 0.4 | 0.46 | 0.45 | 0.09 | 0 | 0.26 | 0.3 | 0.38 | 0.57 | 0.27 | 0.296 |
| Lex - WorryWords | 0.5 | Previous-Sentences-2-Lex-EmoLex | 0.1 | 0.1 | 0.19 | 0.26 | 0.28 | 0.36 | 0.33 | 0.33 | 0.23 | 0.34 | 0.4 | 0.47 | 0.44 | 0.08 | 0 | 0.26 | 0.3 | 0.38 | 0.58 | 0.27 | 0.294 |
| Lex - WorryWords | 0.5 | Previous-Sentences-2-Lex-LIWC-22 | 0.1 | 0.13 | 0.19 | 0.25 | 0.3 | 0.36 | 0.32 | 0.34 | 0.24 | 0.34 | 0.4 | 0.46 | 0.45 | 0.08 | 0 | 0.26 | 0.3 | 0.38 | 0.57 | 0.26 | 0.296 |
| Lex - WorryWords | 0.5 | Previous-Sentences-2-Lex-eMFD | 0.1 | 0.1 | 0.19 | 0.27 | 0.28 | 0.35 | 0.33 | 0.33 | 0.23 | 0.33 | 0.4 | 0.46 | 0.44 | 0.08 | 0 | 0.26 | 0.3 | 0.39 | 0.57 | 0.26 | 0.293 |
| Lex - LIWC 15 | 0.5 | Baseline | 0.5 | 0.09 | 0.21 | 0.23 | 0.28 | 0.34 | 0.3 | 0.36 | 0.24 | 0.31 | 0.42 | 0.45 | 0.43 | 0.11 | 0 | 0.2 | 0.28 | 0.39 | 0.58 | 0.2 | 0.285 |
| Lex - LIWC 15 | 0.5 | Lex-LIWC-22_LingFeat | 0.5 | 0.09 | 0.2 | 0.24 | 0.3 | 0.35 | 0.3 | 0.36 | 0.24 | 0.31 | 0.42 | 0.47 | 0.43 | 0.11 | 0 | 0.2 | 0.28 | 0.39 | 0.58 | 0.19 | 0.286 |
| Lex - LIWC 15 | 0.5 | Lex-LIWC-22_LingFeat | 0.1 | 0.09 | 0.21 | 0.24 | 0.29 | 0.35 | 0.3 | 0.35 | 0.25 | 0.31 | 0.4 | 0.46 | 0.43 | 0.11 | 0 | 0.21 | 0.28 | 0.39 | 0.57 | 0.2 | 0.286 |
| Lex - LIWC 15 | 0.5 | Previous-Sentences-2-Lex-EmoLex | 0.1 | 0.09 | 0.21 | 0.24 | 0.27 | 0.35 | 0.31 | 0.35 | 0.27 | 0.31 | 0.4 | 0.46 | 0.42 | 0.11 | 0 | 0.21 | 0.29 | 0.4 | 0.57 | 0.21 | 0.286 |
| Lex - LIWC 15 | 0.5 | Previous-Sentences-2-Lex-LIWC-22 | 0.1 | 0.1 | 0.21 | 0.23 | 0.3 | 0.35 | 0.3 | 0.36 | 0.27 | 0.3 | 0.4 | 0.45 | 0.42 | 0.1 | 0 | 0.21 | 0.28 | 0.39 | 0.56 | 0.2 | 0.288 |
| Lex - LIWC 15 | 0.5 | Previous-Sentences-2-Lex-eMFD | 0.1 | 0.09 | 0.2 | 0.25 | 0.27 | 0.34 | 0.31 | 0.35 | 0.26 | 0.3 | 0.4 | 0.45 | 0.42 | 0.1 | 0 | 0.21 | 0.29 | 0.4 | 0.57 | 0.2 | 0.286 |
| Lex - LIWC 22 | 0.5 | Baseline | 0.5 | 0.11 | 0.21 | 0.26 | 0.31 | 0.34 | 0.34 | 0.36 | 0.17 | 0.33 | 0.41 | 0.47 | 0.44 | 0.07 | 0 | 0.23 | 0.3 | 0.4 | 0.57 | 0.18 | 0.289 |
| Lex - LIWC 22 | 0.5 | Lex-LIWC-22_LingFeat | 0.5 | 0.1 | 0.21 | 0.27 | 0.29 | 0.35 | 0.33 | 0.35 | 0.18 | 0.33 | 0.41 | 0.49 | 0.44 | 0.07 | 0 | 0.23 | 0.31 | 0.39 | 0.58 | 0.19 | 0.29 |
| Lex - LIWC 22 | 0.5 | Lex-LIWC-22_LingFeat | 0.1 | 0.11 | 0.22 | 0.27 | 0.32 | 0.36 | 0.33 | 0.36 | 0.2 | 0.32 | 0.4 | 0.48 | 0.44 | 0.07 | 0 | 0.25 | 0.31 | 0.39 | 0.57 | 0.2 | 0.295 |
| Lex - LIWC 22 | 0.5 | Previous-Sentences-2-Lex-EmoLex | 0.1 | 0.1 | 0.22 | 0.27 | 0.29 | 0.36 | 0.34 | 0.36 | 0.2 | 0.32 | 0.4 | 0.49 | 0.43 | 0.06 | 0 | 0.25 | 0.3 | 0.4 | 0.57 | 0.2 | 0.292 |
| Lex - LIWC 22 | 0.5 | Previous-Sentences-2-Lex-LIWC-22 | 0.1 | 0.12 | 0.22 | 0.26 | 0.33 | 0.36 | 0.34 | 0.37 | 0.2 | 0.32 | 0.4 | 0.47 | 0.43 | 0.06 | 0 | 0.25 | 0.3 | 0.4 | 0.56 | 0.2 | 0.295 |
| Lex - LIWC 22 | 0.5 | Previous-Sentences-2-Lex-eMFD | 0.1 | 0.09 | 0.22 | 0.28 | 0.29 | 0.35 | 0.34 | 0.36 | 0.18 | 0.32 | 0.4 | 0.48 | 0.43 | 0.06 | 0 | 0.25 | 0.31 | 0.4 | 0.56 | 0.19 | 0.29 |
| Lex - MFD-20 | 0.5 | Baseline | 0.5 | 0.07 | 0.18 | 0.22 | 0.26 | 0.34 | 0.3 | 0.33 | 0.18 | 0.33 | 0.4 | 0.47 | 0.44 | 0.11 | 0 | 0.22 | 0.27 | 0.38 | 0.56 | 0.27 | 0.281 |
| Lex - MFD-20 | 0.5 | Lex-LIWC-22_LingFeat | 0.5 | 0.07 | 0.18 | 0.24 | 0.27 | 0.35 | 0.29 | 0.32 | 0.19 | 0.34 | 0.41 | 0.49 | 0.43 | 0.1 | 0 | 0.21 | 0.29 | 0.38 | 0.56 | 0.26 | 0.283 |
| Lex - MFD-20 | 0.5 | Lex-LIWC-22_LingFeat | 0.1 | 0.09 | 0.2 | 0.23 | 0.28 | 0.35 | 0.29 | 0.33 | 0.21 | 0.32 | 0.39 | 0.49 | 0.43 | 0.11 | 0 | 0.22 | 0.28 | 0.38 | 0.55 | 0.28 | 0.286 |
| Lex - MFD-20 | 0.5 | Previous-Sentences-2-Lex-EmoLex | 0.1 | 0.09 | 0.18 | 0.23 | 0.25 | 0.35 | 0.3 | 0.33 | 0.21 | 0.34 | 0.39 | 0.5 | 0.43 | 0.11 | 0 | 0.22 | 0.28 | 0.39 | 0.56 | 0.28 | 0.286 |
| Lex - MFD-20 | 0.5 | Previous-Sentences-2-Lex-LIWC-22 | 0.1 | 0.1 | 0.19 | 0.23 | 0.29 | 0.35 | 0.29 | 0.33 | 0.21 | 0.34 | 0.39 | 0.49 | 0.43 | 0.11 | 0 | 0.22 | 0.28 | 0.39 | 0.55 | 0.28 | 0.288 |
| Lex - MFD-20 | 0.5 | Previous-Sentences-2-Lex-eMFD | 0.1 | 0.07 | 0.19 | 0.24 | 0.26 | 0.35 | 0.3 | 0.32 | 0.21 | 0.33 | 0.39 | 0.49 | 0.43 | 0.11 | 0 | 0.22 | 0.29 | 0.39 | 0.55 | 0.28 | 0.285 |
| Lex - eMFD | 0.5 | Baseline | 0.5 | 0.08 | 0.18 | 0.22 | 0.27 | 0.34 | 0.29 | 0.33 | 0.18 | 0.33 | 0.41 | 0.49 | 0.44 | 0.11 | 0 | 0.22 | 0.27 | 0.38 | 0.57 | 0.27 | 0.283 |
| Lex - eMFD | 0.5 | Lex-LIWC-22_LingFeat | 0.5 | 0.07 | 0.18 | 0.24 | 0.27 | 0.35 | 0.28 | 0.32 | 0.19 | 0.34 | 0.41 | 0.51 | 0.43 | 0.1 | 0 | 0.21 | 0.29 | 0.38 | 0.57 | 0.26 | 0.284 |
| Lex - eMFD | 0.5 | Lex-LIWC-22_LingFeat | 0.1 | 0.09 | 0.19 | 0.23 | 0.28 | 0.35 | 0.29 | 0.32 | 0.21 | 0.32 | 0.39 | 0.5 | 0.43 | 0.11 | 0 | 0.22 | 0.28 | 0.38 | 0.56 | 0.27 | 0.287 |
| Lex - eMFD | 0.5 | Previous-Sentences-2-Lex-EmoLex | 0.1 | 0.09 | 0.18 | 0.24 | 0.25 | 0.35 | 0.29 | 0.32 | 0.21 | 0.34 | 0.4 | 0.5 | 0.42 | 0.11 | 0 | 0.22 | 0.28 | 0.39 | 0.57 | 0.28 | 0.287 |
| Lex - eMFD | 0.5 | Previous-Sentences-2-Lex-LIWC-22 | 0.1 | 0.1 | 0.18 | 0.23 | 0.3 | 0.35 | 0.29 | 0.33 | 0.22 | 0.34 | 0.4 | 0.5 | 0.43 | 0.1 | 0 | 0.21 | 0.28 | 0.39 | 0.56 | 0.28 | 0.289 |
| Lex - eMFD | 0.5 | Previous-Sentences-2-Lex-eMFD | 0.1 | 0.08 | 0.18 | 0.25 | 0.26 | 0.35 | 0.29 | 0.32 | 0.22 | 0.33 | 0.4 | 0.5 | 0.43 | 0.1 | 0 | 0.22 | 0.29 | 0.39 | 0.56 | 0.28 | 0.286 |
| Lex - MJD | 0.5 | Baseline | 0.5 | 0.12 | 0.2 | 0.27 | 0.29 | 0.36 | 0.33 | 0.36 | 0.23 | 0.35 | 0.41 | 0.46 | 0.45 | 0.09 | 0 | 0.26 | 0.27 | 0.38 | 0.57 | 0.24 | 0.297 |
| Lex - MJD | 0.5 | Lex-LIWC-22_LingFeat | 0.5 | 0.11 | 0.21 | 0.28 | 0.29 | 0.37 | 0.33 | 0.35 | 0.24 | 0.36 | 0.41 | 0.49 | 0.44 | 0.07 | 0 | 0.26 | 0.28 | 0.38 | 0.58 | 0.24 | 0.299 |
| Lex - MJD | 0.5 | Lex-LIWC-22_LingFeat | 0.1 | 0.12 | 0.21 | 0.27 | 0.33 | 0.37 | 0.33 | 0.36 | 0.26 | 0.35 | 0.41 | 0.48 | 0.44 | 0.08 | 0 | 0.26 | 0.28 | 0.38 | 0.57 | 0.26 | 0.302 |
| Lex - MJD | 0.5 | Previous-Sentences-2-Lex-EmoLex | 0.1 | 0.12 | 0.2 | 0.28 | 0.29 | 0.36 | 0.34 | 0.36 | 0.26 | 0.36 | 0.4 | 0.48 | 0.43 | 0.08 | 0 | 0.26 | 0.28 | 0.39 | 0.57 | 0.26 | 0.302 |
| Lex - MJD | 0.5 | Previous-Sentences-2-Lex-LIWC-22 | 0.1 | 0.12 | 0.2 | 0.27 | 0.32 | 0.37 | 0.33 | 0.37 | 0.27 | 0.35 | 0.4 | 0.48 | 0.44 | 0.08 | 0 | 0.26 | 0.28 | 0.38 | 0.56 | 0.26 | 0.303 |
| Lex - MJD | 0.5 | Previous-Sentences-2-Lex-eMFD | 0.1 | 0.09 | 0.2 | 0.28 | 0.27 | 0.36 | 0.34 | 0.35 | 0.26 | 0.36 | 0.4 | 0.47 | 0.44 | 0.08 | 0 | 0.27 | 0.29 | 0.39 | 0.56 | 0.25 | 0.298 |
| Baseline | 0.25 | Baseline | 0.5 | 0.16 | 0.2 | 0.26 | 0.29 | 0.35 | 0.33 | 0.39 | 0.24 | 0.34 | 0.4 | 0.49 | 0.43 | 0.1 | 0.06 | 0.25 | 0.28 | 0.4 | 0.54 | 0.25 | 0.304 |
| Baseline | 0.25 | Lex-LIWC-22_LingFeat | 0.5 | 0.17 | 0.21 | 0.28 | 0.29 | 0.36 | 0.33 | 0.38 | 0.24 | 0.35 | 0.41 | 0.51 | 0.43 | 0.1 | 0.06 | 0.26 | 0.29 | 0.4 | 0.55 | 0.26 | 0.309 |
| Baseline | 0.3 | Lex-LIWC-22_LingFeat | 0.1 | 0.16 | 0.21 | 0.27 | 0.32 | 0.35 | 0.32 | 0.37 | 0.24 | 0.34 | 0.4 | 0.49 | 0.42 | 0.09 | 0 | 0.25 | 0.3 | 0.39 | 0.54 | 0.26 | 0.302 |
| Baseline | 0.25 | Previous-Sentences-2-Lex-EmoLex | 0.1 | 0.15 | 0.21 | 0.27 | 0.28 | 0.35 | 0.33 | 0.37 | 0.25 | 0.34 | 0.4 | 0.5 | 0.41 | 0.11 | 0.06 | 0.26 | 0.28 | 0.4 | 0.53 | 0.27 | 0.303 |

Table S7: Hierarchical DeBERTa with presence gate: test F1-scores per moral value (V1–V19), for different thresholds and filter models, and macro-average (Macro-F1). Part 2.

| Name | Thr | Filter | Filter thr | V1 | V2 | V3 | V4 | V5 | V6 | V7 | V8 | V9 | V10 | V11 | V12 | V13 | V14 | V15 | V16 | V17 | V18 | V19 | Macro-F1 |
|---|---|---|---|---|---|---|---|---|---|---|---|---|---|---|---|---|---|---|---|---|---|---|---|
| Baseline | 0.3 | Previous-Sentences-2-Lex-LIWC-22 | 0.1 | 0.16 | 0.21 | 0.27 | 0.32 | 0.35 | 0.33 | 0.37 | 0.26 | 0.34 | 0.4 | 0.49 | 0.42 | 0.08 | 0 | 0.25 | 0.3 | 0.4 | 0.54 | 0.27 | 0.303 |
| Baseline | 0.25 | Previous-Sentences-2-Lex-eMFD | 0.1 | 0.15 | 0.21 | 0.28 | 0.28 | 0.35 | 0.33 | 0.37 | 0.25 | 0.33 | 0.39 | 0.49 | 0.42 | 0.1 | 0.06 | 0.26 | 0.3 | 0.41 | 0.54 | 0.26 | 0.303 |
| 2 prev sentences with label | 0.3 | Baseline | 0.5 | 0.12 | 0.2 | 0.26 | 0.3 | 0.34 | 0.32 | 0.39 | 0.2 | 0.32 | 0.42 | 0.42 | 0.45 | 0.1 | 0.09 | 0.24 | 0.28 | 0.39 | 0.55 | 0.26 | 0.294 |
| 2 prev sentences with label | 0.3 | Lex-LIWC-22_LingFeat | 0.5 | 0.14 | 0.2 | 0.28 | 0.3 | 0.36 | 0.32 | 0.38 | 0.21 | 0.33 | 0.41 | 0.46 | 0.44 | 0.09 | 0 | 0.24 | 0.29 | 0.39 | 0.57 | 0.25 | 0.298 |
| 2 prev sentences with label | 0.35 | Lex-LIWC-22_LingFeat | 0.1 | 0.12 | 0.21 | 0.26 | 0.31 | 0.34 | 0.32 | 0.37 | 0.22 | 0.33 | 0.41 | 0.42 | 0.45 | 0.07 | 0 | 0.24 | 0.28 | 0.4 | 0.57 | 0.26 | 0.293 |
| 2 prev sentences with label | 0.3 | Previous-Sentences-2-Lex-EmoLex | 0.1 | 0.12 | 0.19 | 0.26 | 0.3 | 0.35 | 0.33 | 0.37 | 0.23 | 0.35 | 0.4 | 0.43 | 0.43 | 0.08 | 0 | 0.25 | 0.29 | 0.4 | 0.55 | 0.26 | 0.294 |
| 2 prev sentences with label | 0.3 | Previous-Sentences-2-Lex-LIWC-22 | 0.1 | 0.14 | 0.2 | 0.26 | 0.32 | 0.35 | 0.33 | 0.38 | 0.25 | 0.34 | 0.4 | 0.42 | 0.43 | 0.08 | 0 | 0.25 | 0.3 | 0.4 | 0.55 | 0.26 | 0.298 |
| 2 prev sentences with label | 0.3 | Previous-Sentences-2-Lex-eMFD | 0.1 | 0.1 | 0.2 | 0.28 | 0.31 | 0.34 | 0.34 | 0.37 | 0.23 | 0.34 | 0.41 | 0.43 | 0.43 | 0.08 | 0 | 0.25 | 0.3 | 0.4 | 0.55 | 0.26 | 0.295 |
| Residual Block | 0.25 | Baseline | 0.5 | 0.16 | 0.2 | 0.25 | 0.28 | 0.35 | 0.35 | 0.37 | 0.21 | 0.38 | 0.43 | 0.47 | 0.43 | 0.14 | 0 | 0.24 | 0.29 | 0.4 | 0.56 | 0.28 | 0.304 |
| Residual Block | 0.3 | Lex-LIWC-22_LingFeat | 0.5 | 0.16 | 0.21 | 0.28 | 0.27 | 0.36 | 0.33 | 0.36 | 0.22 | 0.37 | 0.43 | 0.5 | 0.42 | 0.1 | 0 | 0.25 | 0.3 | 0.4 | 0.57 | 0.28 | 0.306 |
| Residual Block | 0.35 | Lex-LIWC-22_LingFeat | 0.1 | 0.15 | 0.22 | 0.27 | 0.31 | 0.35 | 0.33 | 0.36 | 0.22 | 0.37 | 0.41 | 0.48 | 0.42 | 0.1 | 0 | 0.25 | 0.29 | 0.4 | 0.56 | 0.29 | 0.304 |
| Residual Block | 0.3 | Previous-Sentences-2-Lex-EmoLex | 0.1 | 0.15 | 0.21 | 0.27 | 0.27 | 0.36 | 0.34 | 0.36 | 0.24 | 0.38 | 0.41 | 0.48 | 0.41 | 0.1 | 0 | 0.25 | 0.3 | 0.41 | 0.56 | 0.3 | 0.305 |
| Residual Block | 0.35 | Previous-Sentences-2-Lex-LIWC-22 | 0.1 | 0.15 | 0.21 | 0.27 | 0.31 | 0.35 | 0.33 | 0.36 | 0.24 | 0.37 | 0.41 | 0.48 | 0.43 | 0.1 | 0 | 0.24 | 0.29 | 0.4 | 0.56 | 0.29 | 0.306 |
| Residual Block | 0.3 | Previous-Sentences-2-Lex-eMFD | 0.1 | 0.14 | 0.21 | 0.27 | 0.27 | 0.35 | 0.34 | 0.35 | 0.24 | 0.37 | 0.41 | 0.48 | 0.42 | 0.1 | 0 | 0.25 | 0.3 | 0.41 | 0.57 | 0.29 | 0.304 |
| Lex - VAD | 0.25 | Baseline | 0.5 | 0.16 | 0.2 | 0.27 | 0.26 | 0.35 | 0.34 | 0.37 | 0.24 | 0.35 | 0.43 | 0.48 | 0.44 | 0.14 | 0.05 | 0.23 | 0.28 | 0.4 | 0.56 | 0.26 | 0.306 |
| Lex - VAD | 0.25 | Lex-LIWC-22_LingFeat | 0.5 | 0.16 | 0.21 | 0.28 | 0.26 | 0.36 | 0.34 | 0.36 | 0.24 | 0.37 | 0.43 | 0.51 | 0.44 | 0.13 | 0.05 | 0.22 | 0.28 | 0.39 | 0.57 | 0.26 | 0.308 |
| Lex - VAD | 0.3 | Lex-LIWC-22_LingFeat | 0.1 | 0.14 | 0.2 | 0.26 | 0.29 | 0.35 | 0.33 | 0.36 | 0.24 | 0.35 | 0.41 | 0.49 | 0.44 | 0.13 | 0.05 | 0.23 | 0.29 | 0.39 | 0.55 | 0.26 | 0.303 |
| Lex - VAD | 0.3 | Previous-Sentences-2-Lex-EmoLex | 0.1 | 0.14 | 0.2 | 0.26 | 0.25 | 0.35 | 0.34 | 0.37 | 0.25 | 0.36 | 0.41 | 0.5 | 0.43 | 0.13 | 0.05 | 0.22 | 0.29 | 0.4 | 0.56 | 0.25 | 0.303 |
| Lex - VAD | 0.3 | Previous-Sentences-2-Lex-LIWC-22 | 0.1 | 0.14 | 0.2 | 0.26 | 0.29 | 0.35 | 0.33 | 0.37 | 0.26 | 0.36 | 0.41 | 0.49 | 0.44 | 0.13 | 0.05 | 0.22 | 0.28 | 0.4 | 0.56 | 0.26 | 0.305 |
| Lex - VAD | 0.3 | Previous-Sentences-2-Lex-eMFD | 0.1 | 0.12 | 0.2 | 0.27 | 0.26 | 0.35 | 0.34 | 0.36 | 0.25 | 0.36 | 0.41 | 0.48 | 0.44 | 0.13 | 0.05 | 0.23 | 0.29 | 0.41 | 0.56 | 0.25 | 0.303 |
| Lex - EmoLex | 0.25 | Baseline | 0.5 | 0.1 | 0.19 | 0.27 | 0.29 | 0.36 | 0.33 | 0.39 | 0.24 | 0.33 | 0.42 | 0.44 | 0.44 | 0.12 | 0 | 0.24 | 0.3 | 0.41 | 0.56 | 0.28 | 0.301 |
| Lex - EmoLex | 0.25 | Lex-LIWC-22_LingFeat | 0.5 | 0.1 | 0.2 | 0.28 | 0.3 | 0.37 | 0.33 | 0.38 | 0.25 | 0.34 | 0.43 | 0.47 | 0.44 | 0.11 | 0 | 0.24 | 0.3 | 0.41 | 0.58 | 0.27 | 0.305 |
| Lex - EmoLex | 0.25 | Lex-LIWC-22_LingFeat | 0.1 | 0.11 | 0.2 | 0.26 | 0.31 | 0.36 | 0.33 | 0.37 | 0.25 | 0.33 | 0.41 | 0.44 | 0.43 | 0.11 | 0 | 0.24 | 0.3 | 0.41 | 0.56 | 0.28 | 0.300 |
| Lex - EmoLex | 0.25 | Previous-Sentences-2-Lex-EmoLex | 0.1 | 0.1 | 0.2 | 0.27 | 0.28 | 0.36 | 0.33 | 0.38 | 0.26 | 0.34 | 0.41 | 0.46 | 0.42 | 0.11 | 0 | 0.24 | 0.29 | 0.41 | 0.56 | 0.29 | 0.301 |
| Lex - EmoLex | 0.25 | Previous-Sentences-2-Lex-LIWC-22 | 0.1 | 0.11 | 0.2 | 0.27 | 0.31 | 0.36 | 0.33 | 0.38 | 0.27 | 0.33 | 0.41 | 0.46 | 0.43 | 0.11 | 0 | 0.24 | 0.3 | 0.41 | 0.56 | 0.28 | 0.304 |
| Lex - EmoLex | 0.25 | Previous-Sentences-2-Lex-eMFD | 0.1 | 0.09 | 0.2 | 0.28 | 0.29 | 0.35 | 0.34 | 0.37 | 0.26 | 0.33 | 0.41 | 0.46 | 0.43 | 0.11 | 0 | 0.24 | 0.31 | 0.41 | 0.57 | 0.28 | 0.302 |
| Lex - Emotion Intensity | 0.25 | Baseline | 0.5 | 0.11 | 0.21 | 0.25 | 0.27 | 0.34 | 0.33 | 0.36 | 0.21 | 0.32 | 0.41 | 0.48 | 0.43 | 0.16 | 0 | 0.21 | 0.28 | 0.38 | 0.55 | 0.24 | 0.292 |
| Lex - Emotion Intensity | 0.25 | Lex-LIWC-22_LingFeat | 0.5 | 0.11 | 0.21 | 0.27 | 0.27 | 0.35 | 0.33 | 0.36 | 0.22 | 0.33 | 0.42 | 0.49 | 0.43 | 0.15 | 0 | 0.21 | 0.28 | 0.38 | 0.56 | 0.23 | 0.294 |
| Lex - Emotion Intensity | 0.55 | Lex-LIWC-22_LingFeat | 0.1 | 0.07 | 0.22 | 0.26 | 0.28 | 0.34 | 0.31 | 0.35 | 0.22 | 0.33 | 0.4 | 0.47 | 0.43 | 0.12 | 0 | 0.22 | 0.29 | 0.38 | 0.55 | 0.26 | 0.290 |
| Lex - Emotion Intensity | 0.25 | Previous-Sentences-2-Lex-EmoLex | 0.1 | 0.1 | 0.21 | 0.26 | 0.24 | 0.35 | 0.33 | 0.35 | 0.24 | 0.33 | 0.4 | 0.47 | 0.42 | 0.15 | 0 | 0.22 | 0.29 | 0.38 | 0.54 | 0.25 | 0.291 |
| Lex - Emotion Intensity | 0.5 | Previous-Sentences-2-Lex-LIWC-22 | 0.1 | 0.1 | 0.21 | 0.26 | 0.28 | 0.34 | 0.32 | 0.36 | 0.23 | 0.33 | 0.4 | 0.48 | 0.43 | 0.12 | 0 | 0.21 | 0.28 | 0.38 | 0.55 | 0.25 | 0.291 |
| Lex - Emotion Intensity | 0.25 | Previous-Sentences-2-Lex-eMFD | 0.1 | 0.08 | 0.21 | 0.26 | 0.25 | 0.34 | 0.33 | 0.34 | 0.23 | 0.32 | 0.4 | 0.47 | 0.42 | 0.15 | 0 | 0.22 | 0.3 | 0.38 | 0.54 | 0.25 | 0.290 |
| Lex - WorryWords | 0.35 | Baseline | 0.5 | 0.12 | 0.21 | 0.27 | 0.27 | 0.36 | 0.33 | 0.35 | 0.23 | 0.35 | 0.41 | 0.45 | 0.44 | 0.12 | 0 | 0.25 | 0.29 | 0.4 | 0.56 | 0.26 | 0.299 |
| Lex - WorryWords | 0.25 | Lex-LIWC-22_LingFeat | 0.5 | 0.15 | 0.2 | 0.27 | 0.26 | 0.37 | 0.34 | 0.36 | 0.25 | 0.36 | 0.42 | 0.5 | 0.44 | 0.13 | 0.05 | 0.25 | 0.3 | 0.41 | 0.57 | 0.26 | 0.309 |
| Lex - WorryWords | 0.4 | Lex-LIWC-22_LingFeat | 0.1 | 0.11 | 0.21 | 0.26 | 0.31 | 0.36 | 0.32 | 0.34 | 0.24 | 0.34 | 0.4 | 0.46 | 0.44 | 0.11 | 0 | 0.26 | 0.3 | 0.39 | 0.55 | 0.28 | 0.300 |
| Lex - WorryWords | 0.4 | Previous-Sentences-2-Lex-EmoLex | 0.1 | 0.1 | 0.21 | 0.27 | 0.26 | 0.36 | 0.33 | 0.34 | 0.24 | 0.35 | 0.4 | 0.47 | 0.44 | 0.1 | 0 | 0.26 | 0.3 | 0.4 | 0.56 | 0.28 | 0.299 |
| Lex - WorryWords | 0.4 | Previous-Sentences-2-Lex-LIWC-22 | 0.1 | 0.13 | 0.21 | 0.26 | 0.3 | 0.36 | 0.33 | 0.35 | 0.26 | 0.35 | 0.4 | 0.47 | 0.44 | 0.1 | 0 | 0.25 | 0.3 | 0.39 | 0.55 | 0.28 | 0.301 |
| Lex - WorryWords | 0.3 | Previous-Sentences-2-Lex-eMFD | 0.1 | 0.13 | 0.2 | 0.27 | 0.26 | 0.35 | 0.34 | 0.35 | 0.25 | 0.35 | 0.41 | 0.48 | 0.44 | 0.11 | 0 | 0.26 | 0.3 | 0.41 | 0.55 | 0.27 | 0.303 |
| Lex - LIWC 15 | 0.2 | Baseline | 0.5 | 0.12 | 0.2 | 0.24 | 0.28 | 0.34 | 0.33 | 0.37 | 0.24 | 0.33 | 0.42 | 0.45 | 0.44 | 0.14 | 0.07 | 0.23 | 0.27 | 0.38 | 0.56 | 0.22 | 0.296 |
| Lex - LIWC 15 | 0.2 | Lex-LIWC-22_LingFeat | 0.5 | 0.14 | 0.21 | 0.25 | 0.28 | 0.35 | 0.33 | 0.37 | 0.25 | 0.33 | 0.42 | 0.47 | 0.43 | 0.14 | 0.04 | 0.22 | 0.27 | 0.38 | 0.57 | 0.21 | 0.298 |
| Lex - LIWC 15 | 0.35 | Lex-LIWC-22_LingFeat | 0.1 | 0.1 | 0.21 | 0.24 | 0.3 | 0.34 | 0.31 | 0.36 | 0.25 | 0.32 | 0.4 | 0.45 | 0.44 | 0.13 | 0 | 0.21 | 0.27 | 0.39 | 0.57 | 0.24 | 0.291 |
| Lex - LIWC 15 | 0.2 | Previous-Sentences-2-Lex-EmoLex | 0.1 | 0.12 | 0.2 | 0.25 | 0.26 | 0.34 | 0.32 | 0.36 | 0.25 | 0.33 | 0.4 | 0.45 | 0.42 | 0.13 | 0.04 | 0.22 | 0.27 | 0.38 | 0.55 | 0.23 | 0.291 |
| Lex - LIWC 15 | 0.35 | Previous-Sentences-2-Lex-LIWC-22 | 0.1 | 0.11 | 0.21 | 0.24 | 0.32 | 0.35 | 0.31 | 0.37 | 0.27 | 0.32 | 0.4 | 0.45 | 0.43 | 0.12 | 0 | 0.21 | 0.28 | 0.4 | 0.56 | 0.24 | 0.295 |
| Lex - LIWC 15 | 0.25 | Previous-Sentences-2-Lex-eMFD | 0.1 | 0.11 | 0.21 | 0.26 | 0.27 | 0.34 | 0.32 | 0.35 | 0.26 | 0.32 | 0.4 | 0.45 | 0.43 | 0.14 | 0.08 | 0.23 | 0.28 | 0.4 | 0.55 | 0.24 | 0.297 |
| Lex - LIWC 22 | 0.35 | Baseline | 0.5 | 0.13 | 0.22 | 0.26 | 0.3 | 0.35 | 0.33 | 0.38 | 0.19 | 0.33 | 0.42 | 0.48 | 0.43 | 0.11 | 0.06 | 0.24 | 0.3 | 0.41 | 0.56 | 0.22 | 0.301 |
| Lex - LIWC 22 | 0.25 | Lex-LIWC-22_LingFeat | 0.5 | 0.15 | 0.21 | 0.28 | 0.3 | 0.36 | 0.33 | 0.39 | 0.19 | 0.35 | 0.43 | 0.5 | 0.43 | 0.14 | 0.06 | 0.23 | 0.3 | 0.4 | 0.56 | 0.23 | 0.307 |
| Lex - LIWC 22 | 0.4 | Lex-LIWC-22_LingFeat | 0.1 | 0.12 | 0.22 | 0.26 | 0.31 | 0.36 | 0.33 | 0.37 | 0.21 | 0.32 | 0.41 | 0.48 | 0.43 | 0.08 | 0.06 | 0.25 | 0.3 | 0.4 | 0.56 | 0.22 | 0.299 |
| Lex - LIWC 22 | 0.35 | Previous-Sentences-2-Lex-EmoLex | 0.1 | 0.12 | 0.22 | 0.27 | 0.28 | 0.36 | 0.33 | 0.37 | 0.22 | 0.33 | 0.41 | 0.49 | 0.42 | 0.1 | 0.06 | 0.25 | 0.3 | 0.41 | 0.56 | 0.23 | 0.301 |
| Lex - LIWC 22 | 0.4 | Previous-Sentences-2-Lex-LIWC-22 | 0.1 | 0.12 | 0.22 | 0.26 | 0.33 | 0.36 | 0.33 | 0.37 | 0.22 | 0.32 | 0.41 | 0.48 | 0.43 | 0.07 | 0.06 | 0.24 | 0.29 | 0.4 | 0.56 | 0.23 | 0.301 |
| Lex - LIWC 22 | 0.35 | Previous-Sentences-2-Lex-eMFD | 0.1 | 0.11 | 0.22 | 0.28 | 0.27 | 0.35 | 0.33 | 0.36 | 0.21 | 0.32 | 0.41 | 0.49 | 0.43 | 0.09 | 0.06 | 0.25 | 0.31 | 0.41 | 0.56 | 0.22 | 0.299 |
| Lex - MFD-20 | 0.45 | Baseline | 0.5 | 0.07 | 0.18 | 0.22 | 0.25 | 0.34 | 0.3 | 0.34 | 0.19 | 0.33 | 0.4 | 0.47 | 0.44 | 0.11 | 0 | 0.22 | 0.28 | 0.39 | 0.56 | 0.27 | 0.282 |
| Lex - MFD-20 | 0.25 | Lex-LIWC-22_LingFeat | 0.5 | 0.13 | 0.19 | 0.26 | 0.26 | 0.36 | 0.3 | 0.35 | 0.22 | 0.31 | 0.41 | 0.51 | 0.44 | 0.12 | 0.05 | 0.25 | 0.3 | 0.38 | 0.56 | 0.27 | 0.300 |
| Lex - MFD-20 | 0.45 | Lex-LIWC-22_LingFeat | 0.1 | 0.09 | 0.19 | 0.23 | 0.27 | 0.35 | 0.29 | 0.34 | 0.21 | 0.32 | 0.39 | 0.48 | 0.44 | 0.11 | 0 | 0.22 | 0.28 | 0.38 | 0.56 | 0.27 | 0.286 |
| Lex - MFD-20 | 0.45 | Previous-Sentences-2-Lex-EmoLex | 0.1 | 0.09 | 0.18 | 0.23 | 0.25 | 0.35 | 0.3 | 0.34 | 0.21 | 0.34 | 0.39 | 0.49 | 0.43 | 0.11 | 0 | 0.22 | 0.28 | 0.39 | 0.56 | 0.28 | 0.287 |
| Lex - MFD-20 | 0.45 | Previous-Sentences-2-Lex-LIWC-22 | 0.1 | 0.1 | 0.18 | 0.23 | 0.28 | 0.35 | 0.29 | 0.34 | 0.22 | 0.34 | 0.4 | 0.48 | 0.44 | 0.1 | 0 | 0.22 | 0.28 | 0.39 | 0.56 | 0.28 | 0.288 |
| Lex - MFD-20 | 0.45 | Previous-Sentences-2-Lex-eMFD | 0.1 | 0.07 | 0.18 | 0.24 | 0.26 | 0.35 | 0.3 | 0.34 | 0.22 | 0.33 | 0.39 | 0.49 | 0.43 | 0.1 | 0 | 0.22 | 0.3 | 0.39 | 0.56 | 0.27 | 0.286 |
| Lex - eMFD | 0.3 | Baseline | 0.5 | 0.09 | 0.19 | 0.24 | 0.26 | 0.35 | 0.3 | 0.35 | 0.22 | 0.31 | 0.41 | 0.48 | 0.44 | 0.12 | 0.05 | 0.25 | 0.28 | 0.39 | 0.56 | 0.26 | 0.293 |
| Lex - eMFD | 0.3 | Lex-LIWC-22_LingFeat | 0.5 | 0.09 | 0.2 | 0.25 | 0.27 | 0.35 | 0.3 | 0.34 | 0.22 | 0.33 | 0.42 | 0.5 | 0.44 | 0.11 | 0.05 | 0.24 | 0.29 | 0.39 | 0.57 | 0.26 | 0.295 |
| Lex - eMFD | 0.45 | Lex-LIWC-22_LingFeat | 0.1 | 0.09 | 0.19 | 0.24 | 0.27 | 0.35 | 0.29 | 0.33 | 0.22 | 0.32 | 0.39 | 0.5 | 0.43 | 0.12 | 0.06 | 0.22 | 0.28 | 0.38 | 0.57 | 0.27 | 0.291 |
| Lex - eMFD | 0.4 | Previous-Sentences-2-Lex-EmoLex | 0.1 | 0.09 | 0.19 | 0.24 | 0.25 | 0.35 | 0.3 | 0.34 | 0.24 | 0.34 | 0.4 | 0.51 | 0.42 | 0.11 | 0.06 | 0.22 | 0.28 | 0.4 | 0.56 | 0.29 | 0.294 |
| Lex - eMFD | 0.35 | Previous-Sentences-2-Lex-LIWC-22 | 0.1 | 0.1 | 0.19 | 0.23 | 0.27 | 0.35 | 0.3 | 0.35 | 0.26 | 0.33 | 0.4 | 0.49 | 0.43 | 0.11 | 0.06 | 0.23 | 0.27 | 0.39 | 0.55 | 0.27 | 0.294 |
| Lex - eMFD | 0.35 | Previous-Sentences-2-Lex-eMFD | 0.1 | 0.07 | 0.19 | 0.25 | 0.25 | 0.35 | 0.3 | 0.34 | 0.25 | 0.32 | 0.4 | 0.49 | 0.43 | 0.11 | 0.06 | 0.24 | 0.28 | 0.4 | 0.55 | 0.27 | 0.292 |
| Lex - MJD | 0.2 | Baseline | 0.5 | 0.15 | 0.21 | 0.26 | 0.31 | 0.36 | 0.34 | 0.39 | 0.24 | 0.35 | 0.43 | 0.45 | 0.44 | 0.14 | 0.06 | 0.24 | 0.28 | 0.41 | 0.56 | 0.26 | 0.308 |
| Lex - MJD | 0.2 | Lex-LIWC-22_LingFeat | 0.5 | 0.15 | 0.21 | 0.27 | 0.32 | 0.37 | 0.34 | 0.38 | 0.25 | 0.36 | 0.43 | 0.47 | 0.43 | 0.13 | 0.06 | 0.24 | 0.28 | 0.41 | 0.57 | 0.26 | 0.312 |
| Lex - MJD | 0.4 | Lex-LIWC-22_LingFeat | 0.1 | 0.14 | 0.21 | 0.26 | 0.32 | 0.37 | 0.34 | 0.37 | 0.27 | 0.35 | 0.41 | 0.48 | 0.44 | 0.12 | 0.06 | 0.25 | 0.28 | 0.39 | 0.56 | 0.26 | 0.310 |
| Lex - MJD | 0.3 | Previous-Sentences-2-Lex-EmoLex | 0.1 | 0.14 | 0.21 | 0.27 | 0.28 | 0.36 | 0.35 | 0.38 | 0.26 | 0.36 | 0.42 | 0.49 | 0.43 | 0.12 | 0.06 | 0.24 | 0.29 | 0.42 | 0.56 | 0.29 | 0.312 |
| Lex - MJD | 0.4 | Previous-Sentences-2-Lex-LIWC-22 | 0.1 | 0.15 | 0.21 | 0.27 | 0.31 | 0.36 | 0.35 | 0.38 | 0.29 | 0.35 | 0.41 | 0.48 | 0.44 | 0.12 | 0.06 | 0.25 | 0.29 | 0.39 | 0.56 | 0.26 | 0.313 |
| Lex - MJD | 0.3 | Previous-Sentences-2-Lex-eMFD | 0.1 | 0.13 | 0.21 | 0.27 | 0.28 | 0.36 | 0.35 | 0.37 | 0.27 | 0.36 | 0.42 | 0.48 | 0.44 | 0.13 | 0.06 | 0.24 | 0.3 | 0.41 | 0.56 | 0.28 | 0.311 |

Table S8: LLM-based classifiers: validation F1-scores per moral value (V1–V19) and macro-average (Macro-F1). Moral-value IDs V1–V19 are defined in the moral-value ID mapping table in this section.

| Model | Mode | Prompt | V1 | V2 | V3 | V4 | V5 | V6 | V7 | V8 | V9 | V10 | V11 | V12 | V13 | V14 | V15 | V16 | V17 | V18 | V19 | Macro-F1 |
|---|---|---|---|---|---|---|---|---|---|---|---|---|---|---|---|---|---|---|---|---|---|---|
| meta-llama-Llama-3-1-8B-Instruct | zero-shot | direct | 0.06 | 0.09 | 0.02 | 0.12 | 0.25 | 0.24 | 0.15 | 0.02 | 0.06 | 0.21 | 0.19 | 0.12 | 0 | 0.05 | 0.12 | 0.11 | 0.2 | 0.17 | 0.07 | 0.119 |
| meta-llama-Llama-3-1-8B-Instruct | zero-shot | cot_hidden | 0.06 | 0.12 | 0.04 | 0.09 | 0.27 | 0.21 | 0.15 | 0.03 | 0.05 | 0.19 | 0.07 | 0.17 | 0.02 | 0.03 | 0.08 | 0.06 | 0.13 | 0.11 | 0.04 | 0.100 |
| meta-llama-Llama-3-1-8B-Instruct | zero-shot | definition | 0.06 | 0.14 | 0.11 | 0.1 | 0.24 | 0.22 | 0.16 | 0.17 | 0.14 | 0.26 | 0.21 | 0.22 | 0.05 | 0.02 | 0.13 | 0.09 | 0.24 | 0.43 | 0.08 | 0.163 |
| meta-llama-Llama-3-1-8B-Instruct | zero-shot | qa | 0.04 | 0.1 | 0.02 | 0.09 | 0.25 | 0.23 | 0.17 | 0.01 | 0.05 | 0.19 | 0.08 | 0.17 | 0.02 | 0.01 | 0.09 | 0.07 | 0.14 | 0.08 | 0.04 | 0.097 |
| meta-llama-Llama-3-1-8B-Instruct | few-shot | definition-1 | 0.07 | 0.1 | 0.08 | 0.23 | 0.23 | 0.04 | 0.11 | 0.09 | 0.18 | 0.22 | 0.28 | 0.07 | 0.02 | 0 | 0.15 | 0.07 | 0.28 | 0.41 | 0.04 | 0.141 |
| meta-llama-Llama-3-1-8B-Instruct | few-shot | definition-2 | 0.06 | 0.13 | 0.13 | 0.1 | 0.26 | 0.19 | 0.18 | 0.07 | 0.11 | 0.16 | 0.28 | 0.11 | 0.01 | 0 | 0.19 | 0.09 | 0.2 | 0.44 | 0.05 | 0.146 |
| meta-llama-Llama-3-1-8B-Instruct | few-shot | definition-4 | 0.06 | 0.13 | 0.13 | 0.13 | 0.27 | 0.2 | 0.2 | 0.08 | 0.1 | 0.2 | 0.28 | 0.14 | 0 | 0.01 | 0.19 | 0.11 | 0.2 | 0.46 | 0.07 | 0.156 |
| meta-llama-Llama-3-1-8B-Instruct | few-shot | definition-8 | 0.06 | 0.16 | 0.13 | 0.18 | 0.25 | 0.17 | 0.21 | 0.07 | 0.13 | 0.14 | 0.29 | 0.24 | 0.05 | 0.03 | 0.19 | 0.08 | 0.17 | 0.42 | 0.12 | 0.162 |
| meta-llama-Llama-3-1-8B-Instruct | few-shot | definition-12 | 0.06 | 0.17 | 0.15 | 0.21 | 0.25 | 0.16 | 0.23 | 0.07 | 0.11 | 0.17 | 0.26 | 0.18 | 0.04 | 0.04 | 0.06 | 0.1 | 0.19 | 0.41 | 0.09 | 0.155 |
| meta-llama-Llama-3-1-8B-Instruct | few-shot | definition-16 | 0.06 | 0.15 | 0.15 | 0.18 | 0.26 | 0.19 | 0.23 | 0.06 | 0.13 | 0.25 | 0.29 | 0.23 | 0.04 | 0.03 | 0.06 | 0.09 | 0.22 | 0.46 | 0.13 | 0.169 |
| meta-llama-Llama-3-1-8B-Instruct | few-shot | definition-20 | 0.07 | 0.15 | 0.13 | 0.16 | 0.27 | 0.25 | 0.24 | 0.11 | 0.12 | 0.28 | 0.29 | 0.24 | 0.02 | 0.03 | 0.18 | 0.08 | 0.23 | 0.45 | 0.14 | 0.182 |
| mistralai-Ministral-8B-Instruct-2410 | zero-shot | direct | 0.04 | 0.07 | 0.09 | 0.06 | 0.23 | 0.2 | 0.13 | 0.06 | 0.1 | 0.24 | 0.11 | 0.1 | 0.02 | 0.01 | 0.13 | 0.04 | 0.17 | 0.18 | 0.05 | 0.106 |
| mistralai-Ministral-8B-Instruct-2410 | zero-shot | cot_hidden | 0.04 | 0.07 | 0.08 | 0.05 | 0.19 | 0.15 | 0.12 | 0.05 | 0.07 | 0.2 | 0.06 | 0.13 | 0.03 | 0.01 | 0.09 | 0.02 | 0.12 | 0.13 | 0.03 | 0.087 |
| mistralai-Ministral-8B-Instruct-2410 | zero-shot | definition | 0.05 | 0.09 | 0.13 | 0.09 | 0.29 | 0.26 | 0.19 | 0.17 | 0.15 | 0.3 | 0.26 | 0.27 | 0.08 | 0.04 | 0.21 | 0.1 | 0.2 | 0.39 | 0.07 | 0.177 |
| mistralai-Ministral-8B-Instruct-2410 | zero-shot | qa | 0.05 | 0.07 | 0.09 | 0.07 | 0.21 | 0.18 | 0.15 | 0.06 | 0.08 | 0.23 | 0.09 | 0.13 | 0.03 | 0.01 | 0.11 | 0.03 | 0.15 | 0.18 | 0.03 | 0.102 |
| mistralai-Ministral-8B-Instruct-2410 | few-shot | definition-1 | 0.02 | 0.09 | 0.04 | 0.04 | 0.12 | 0.18 | 0.03 | 0.07 | 0 | 0.06 | 0.09 | 0.1 | 0.02 | 0 | 0.07 | 0 | 0.09 | 0.48 | 0.11 | 0.085 |
| mistralai-Ministral-8B-Instruct-2410 | few-shot | definition-2 | 0.04 | 0.11 | 0.08 | 0.05 | 0.16 | 0.26 | 0.2 | 0.09 | 0.02 | 0.06 | 0.1 | 0.1 | 0 | 0 | 0.12 | 0.04 | 0.11 | 0.38 | 0.11 | 0.107 |
| mistralai-Ministral-8B-Instruct-2410 | few-shot | definition-4 | 0.07 | 0.13 | 0.13 | 0.16 | 0.26 | 0.26 | 0.21 | 0.12 | 0.07 | 0.08 | 0.13 | 0.15 | 0.04 | 0.04 | 0.15 | 0.06 | 0.11 | 0.36 | 0.12 | 0.138 |
| mistralai-Ministral-8B-Instruct-2410 | few-shot | definition-8 | 0.06 | 0.08 | 0.13 | 0.15 | 0.24 | 0.24 | 0.23 | 0.09 | 0.08 | 0.09 | 0.12 | 0.21 | 0.04 | 0 | 0.16 | 0.03 | 0.12 | 0.39 | 0.06 | 0.131 |
| mistralai-Ministral-8B-Instruct-2410 | few-shot | definition-12 | 0.06 | 0.09 | 0.13 | 0.25 | 0.25 | 0.23 | 0.25 | 0.1 | 0.08 | 0.11 | 0.17 | 0.16 | 0.04 | 0 | 0.17 | 0.09 | 0.13 | 0.4 | 0.05 | 0.146 |
| mistralai-Ministral-8B-Instruct-2410 | few-shot | definition-16 | 0.1 | 0.11 | 0.14 | 0.21 | 0.21 | 0.2 | 0.24 | 0.13 | 0.12 | 0.19 | 0.2 | 0.21 | 0.04 | 0 | 0.14 | 0.09 | 0.12 | 0.44 | 0.08 | 0.156 |
| mistralai-Ministral-8B-Instruct-2410 | few-shot | definition-20 | 0.1 | 0.12 | 0.14 | 0.24 | 0.21 | 0.25 | 0.27 | 0.14 | 0.15 | 0.2 | 0.21 | 0.21 | 0.05 | 0 | 0.17 | 0.08 | 0.13 | 0.46 | 0.08 | 0.168 |
| Qwen-Qwen2-5-7B-Instruct | zero-shot | direct | 0.06 | 0.04 | 0.11 | 0.13 | 0.18 | 0.16 | 0.11 | 0.02 | 0.07 | 0.18 | 0.16 | 0.03 | 0 | 0 | 0.09 | 0.07 | 0.08 | 0.21 | 0.01 | 0.091 |
| Qwen-Qwen2-5-7B-Instruct | zero-shot | cot_hidden | 0 | 0.02 | 0.04 | 0.06 | 0.07 | 0.05 | 0.02 | 0.01 | 0.06 | 0.05 | 0.04 | 0 | 0 | 0 | 0.05 | 0.02 | 0.06 | 0.09 | 0 | 0.037 |
| Qwen-Qwen2-5-7B-Instruct | zero-shot | definition | 0 | 0.03 | 0.04 | 0.09 | 0.1 | 0.06 | 0.05 | 0.05 | 0.06 | 0.1 | 0.24 | 0.05 | 0 | 0 | 0.05 | 0 | 0.08 | 0.26 | 0.02 | 0.068 |
| Qwen-Qwen2-5-7B-Instruct | zero-shot | qa | 0.01 | 0.04 | 0.03 | 0.1 | 0.11 | 0.06 | 0.04 | 0.02 | 0.06 | 0.11 | 0.17 | 0.06 | 0 | 0 | 0.06 | 0.02 | 0.09 | 0.17 | 0 | 0.061 |
| Qwen-Qwen2-5-7B-Instruct | few-shot | direct-1 | 0.04 | 0.04 | 0.1 | 0.12 | 0.24 | 0.26 | 0.19 | 0.02 | 0.12 | 0.23 | 0.13 | 0.06 | 0 | 0 | 0.13 | 0.07 | 0.13 | 0.12 | 0.05 | 0.107 |
| Qwen-Qwen2-5-7B-Instruct | few-shot | direct-2 | 0.09 | 0.08 | 0.11 | 0.07 | 0.26 | 0.24 | 0.23 | 0.03 | 0.12 | 0.23 | 0.21 | 0.09 | 0 | 0 | 0.14 | 0.06 | 0.19 | 0.21 | 0.05 | 0.127 |
| Qwen-Qwen2-5-7B-Instruct | few-shot | direct-4 | 0.1 | 0.09 | 0.14 | 0.07 | 0.27 | 0.26 | 0.24 | 0.02 | 0.13 | 0.22 | 0.24 | 0.11 | 0.01 | 0.11 | 0.17 | 0.08 | 0.22 | 0.25 | 0.03 | 0.146 |
| Qwen-Qwen2-5-7B-Instruct | few-shot | direct-8 | 0.06 | 0.14 | 0.14 | 0 | 0.18 | 0.26 | 0.23 | 0.02 | 0.15 | 0.19 | 0.12 | 0.18 | 0.05 | 0 | 0.16 | 0.07 | 0.21 | 0.2 | 0.05 | 0.127 |
| Qwen-Qwen2-5-7B-Instruct | few-shot | direct-12 | 0.07 | 0.15 | 0.13 | 0.18 | 0.23 | 0.29 | 0.24 | 0.02 | 0.1 | 0.17 | 0.35 | 0.2 | 0.06 | 0.07 | 0.13 | 0.02 | 0.23 | 0.2 | 0.06 | 0.152 |
| Qwen-Qwen2-5-7B-Instruct | few-shot | direct-16 | 0.06 | 0.12 | 0.11 | 0.15 | 0.25 | 0.29 | 0.23 | 0.03 | 0.18 | 0.27 | 0.36 | 0.19 | 0.07 | 0.13 | 0.09 | 0.04 | 0.21 | 0.33 | 0.07 | 0.169 |
| Qwen-Qwen2-5-7B-Instruct | few-shot | direct-20 | 0.07 | 0.13 | 0.11 | 0.15 | 0.24 | 0.32 | 0.25 | 0.09 | 0.17 | 0.3 | 0.37 | 0.19 | 0.07 | 0 | 0.13 | 0.04 | 0.24 | 0.36 | 0.09 | 0.175 |
| google-gemma-2-9b-it | zero-shot | direct | 0.08 | 0.17 | 0.12 | 0.32 | 0.3 | 0.28 | 0.25 | 0.16 | 0.13 | 0.19 | 0.35 | 0.23 | 0.05 | 0.04 | 0.22 | 0.01 | 0.27 | 0.22 | 0.09 | 0.184 |
| google-gemma-2-9b-it | zero-shot | cot_hidden | 0.07 | 0.17 | 0.13 | 0.31 | 0.32 | 0.26 | 0.25 | 0.16 | 0.15 | 0.19 | 0.28 | 0.21 | 0.05 | 0 | 0.21 | 0.02 | 0.25 | 0.31 | 0.11 | 0.182 |
| google-gemma-2-9b-it | zero-shot | definition | 0.09 | 0.19 | 0.19 | 0.27 | 0.3 | 0.29 | 0.24 | 0.18 | 0.18 | 0.25 | 0.23 | 0.29 | 0.07 | 0.04 | 0.24 | 0.05 | 0.32 | 0.55 | 0.12 | 0.215 |
| google-gemma-2-9b-it | zero-shot hier (SBERT gate) | definition | 0.09 | 0.19 | 0.22 | 0.24 | 0.31 | 0.29 | 0.24 | 0.2 | 0.2 | 0.27 | 0.24 | 0.3 | 0.08 | 0.04 | 0.24 | 0.05 | 0.32 | 0.57 | 0.13 | 0.223 |
| google-gemma-2-9b-it | zero-shot | qa | 0.07 | 0.17 | 0.11 | 0.32 | 0.32 | 0.27 | 0.26 | 0.13 | 0.17 | 0.19 | 0.34 | 0.22 | 0.05 | 0 | 0.2 | 0.02 | 0.26 | 0.16 | 0.08 | 0.176 |
| google-gemma-2-9b-it | few-shot | definition-1 | 0.1 | 0.13 | 0.15 | 0.22 | 0.32 | 0.3 | 0.24 | 0.18 | 0.2 | 0.31 | 0.34 | 0.28 | 0.08 | 0 | 0.25 | 0.03 | 0.22 | 0.4 | 0.12 | 0.204 |
| google-gemma-2-9b-it | few-shot | definition-2 | 0.1 | 0.12 | 0.13 | 0.26 | 0.3 | 0.3 | 0.29 | 0.17 | 0.16 | 0.28 | 0.31 | 0.3 | 0.07 | 0 | 0.26 | 0.02 | 0.27 | 0.52 | 0.1 | 0.209 |
| google-gemma-2-9b-it | few-shot | definition-4 | 0.11 | 0.16 | 0.13 | 0.32 | 0.31 | 0.3 | 0.28 | 0.17 | 0.15 | 0.28 | 0.32 | 0.3 | 0.09 | 0 | 0.26 | 0.03 | 0.29 | 0.52 | 0.09 | 0.215 |
| google-gemma-2-9b-it | few-shot | definition-8 | 0.09 | 0.13 | 0.12 | 0.29 | 0.3 | 0.29 | 0.27 | 0.15 | 0.15 | 0.28 | 0.36 | 0.3 | 0.09 | 0 | 0.23 | 0 | 0.29 | 0.48 | 0.18 | 0.210 |
| google-gemma-2-9b-it | few-shot | definition-12 | 0.1 | 0.13 | 0.15 | 0.29 | 0.29 | 0.29 | 0.26 | 0.14 | 0.12 | 0.26 | 0.32 | 0.28 | 0.09 | 0.04 | 0.24 | 0.01 | 0.26 | 0.37 | 0.18 | 0.201 |
| google-gemma-2-9b-it | few-shot | definition-16 | 0.08 | 0.15 | 0.15 | 0.31 | 0.32 | 0.28 | 0.26 | 0.12 | 0.13 | 0.33 | 0.32 | 0.28 | 0.09 | 0 | 0.24 | 0.01 | 0.28 | 0.54 | 0.19 | 0.215 |
| google-gemma-2-9b-it | few-shot | definition-20 | 0.08 | 0.15 | 0.16 | 0.31 | 0.32 | 0.33 | 0.27 | 0.19 | 0.12 | 0.34 | 0.35 | 0.29 | 0.1 | 0 | 0.26 | 0.01 | 0.27 | 0.54 | 0.16 | 0.225 |
| google-gemma-2-9b-it | few-shot hier (SBERT gate) | definition-20 | 0.09 | 0.15 | 0.18 | 0.3 | 0.32 | 0.33 | 0.27 | 0.21 | 0.13 | 0.34 | 0.37 | 0.3 | 0.1 | 0 | 0.26 | 0.01 | 0.28 | 0.58 | 0.17 | 0.232 |
| google-gemma-2-9b-it | QLoRA direct | definition | 0.02 | 0.17 | 0.24 | 0.27 | 0.33 | 0.28 | 0.28 | 0.24 | 0.33 | 0.46 | 0.4 | 0.46 | 0.04 | 0.07 | 0.19 | 0.21 | 0.02 | 0.21 | 0.14 | 0.231 |
| google-gemma-2-9b-it | QLoRA hier (SBERT gate) | definition | - | - | - | - | - | - | - | - | - | - | - | - | - | - | - | - | - | - | - | - |

Table S9: LLM-based classifiers: test F1-scores per moral value (V1–V19) and macro-average (Macro-F1). Moral-value IDs V1–V19 are defined in the moral-value ID mapping table in this section.

| **Model** | **Mode** | **Prompt** | **V1** | **V2** | **V3** | **V4** | **V5** | **V6** | **V7** | **V8** | **V9** | **V10** | **V11** | **V12** | **V13** | **V14** | **V15** | **V16** | **V17** | **V18** | **V19** | **Macro-F1** |
|---|---|---|---|---|---|---|---|---|---|---|---|---|---|---|---|---|---|---|---|---|---|---|
| google-gemma-2-9b-it | zero-shot | definition | 0.15 | 0.17 | 0.12 | 0.28 | 0.29 | 0.25 | 0.21 | 0.17 | 0.25 | 0.26 | 0.31 | 0.3 | 0.06 | 0.06 | 0.25 | 0.06 | 0.37 | 0.53 | 0.11 | 0.221 |
| google-gemma-2-9b-it | zero-shot hier (SBERT gate) | definition | 0.15 | 0.16 | 0.13 | 0.28 | 0.3 | 0.25 | 0.21 | 0.19 | 0.27 | 0.28 | 0.35 | 0.32 | 0.07 | 0.06 | 0.26 | 0.06 | 0.37 | 0.53 | 0.11 | 0.229 |
| google-gemma-2-9b-it | few-shot | definition-20 | 0.15 | 0.18 | 0.11 | 0.27 | 0.29 | 0.25 | 0.29 | 0.21 | 0.21 | 0.34 | 0.38 | 0.27 | 0.09 | 0.06 | 0.24 | 0.01 | 0.36 | 0.51 | 0.19 | 0.233 |
| google-gemma-2-9b-it | few-shot hier (SBERT gate) | definition-20 | 0.14 | 0.17 | 0.14 | 0.27 | 0.29 | 0.24 | 0.29 | 0.21 | 0.22 | 0.35 | 0.41 | 0.28 | 0.09 | 0.06 | 0.24 | 0.01 | 0.36 | 0.51 | 0.19 | 0.238 |
| google-gemma-2-9b-it | QLoRA direct | definition | 0.07 | 0.16 | 0.15 | 0.31 | 0.32 | 0.26 | 0.35 | 0.23 | 0.34 | 0.44 | 0.53 | 0.45 | 0.05 | 0.06 | 0.19 | 0.2 | 0.04 | 0.29 | 0.06 | 0.236 |
| google-gemma-2-9b-it | QLoRA hier (SBERT gate) | definition | - | - | - | - | - | - | - | - | - | - | - | - | - | - | - | - | - | - | - | - |

Table S10: Ensemble configurations based on transformer architectures (direct and presence) and the applied filters, and their macro-average F1 on the validation and test sets. Part 1.

| Architecture | Models | Dataset | Mode | Threshold | Macro-F1 |
|---|---|---|---|---|---|
| Direct | Lex-LIWC-22-val.tsv | Validation | — | 0.50 | 0.288 |
| Direct | ['Lex-LIWC-22-val.tsv', 'Previous-Sentences-2-val.tsv'] | Validation | hard | 0.50 | 0.315 |
| Direct | Lex-LIWC-22-val.tsv | Validation | weighted | 0.50 | 0.288 |
| Direct | Lex-LIWC-22-val.tsv | Validation | soft | 0.50 | 0.288 |
| Direct | Previous-Sentences-2-val.tsv | Validation | — | 0.30 | 0.315 |
| Direct | Previous-Sentences-2-val.tsv | Validation | hard | Tuned | 0.315 |
| Direct | Lex-LIWC-22-val.tsv | Validation | weighted | Tuned | 0.288 |
| Direct | ['Lex-LIWC-22-val.tsv', 'Previous-Sentences-2-val.tsv', 'Baseline-val.tsv'] | Validation | soft | 0.30 | 0.326 |
| Direct | ['Lex-LIWC-22-test.tsv', 'Previous-Sentences-2-test.tsv', 'Baseline-test.tsv'] | Test | — | 0.50 | 0.286 |
| Direct | ['Lex-LIWC-22-test.tsv', 'Previous-Sentences-2-test.tsv', 'Baseline-test.tsv'] | Test | hard | 0.50 | 0.285 |
| Direct | ['Lex-LIWC-22-test.tsv', 'Previous-Sentences-2-test.tsv', 'Baseline-test.tsv'] | Test | weighted | 0.50 | 0.287 |
| Direct | ['Lex-LIWC-22-test.tsv', 'Previous-Sentences-2-test.tsv', 'Baseline-test.tsv'] | Test | soft | 0.50 | 0.287 |
| Direct | ['Lex-LIWC-22-test.tsv', 'Previous-Sentences-2-test.tsv', 'Baseline-test.tsv'] | Test | — | 0.30 | 0.322 |
| Direct | ['Lex-LIWC-22-test.tsv', 'Previous-Sentences-2-test.tsv', 'Baseline-test.tsv'] | Test | hard | Tuned | 0.324 |
| Direct | ['Lex-LIWC-22-test.tsv', 'Previous-Sentences-2-test.tsv', 'Baseline-test.tsv'] | Test | weighted | Tuned | 0.287 |
| Direct | ['Lex-LIWC-22-test.tsv', 'Previous-Sentences-2-test.tsv', 'Baseline-test.tsv'] | Test | soft | 0.30 | 0.328 |
| Presence | 1_Baseline_0.5_Previous-Sentences-2-val.tsv | Validation | — | 0.50 | 0.293 |
| Presence | ['1_Baseline_0.5_Previous-Sentences-2-val.tsv', '1_Baseline_0.5_Lex-MJD-val.tsv'] | Validation | hard | 0.50 | 0.309 |
| Presence | 1_Baseline_0.5_Previous-Sentences-2-val.tsv | Validation | weighted | 0.50 | 0.293 |
| Presence | 1_Baseline_0.5_Previous-Sentences-2-val.tsv | Validation | soft | 0.50 | 0.293 |
| Presence | 1_Baseline_0.5_Lex-EmoLex-val.tsv | Validation | — | 0.25 | 0.304 |
| Presence | 1_Baseline_0.5_Lex-EmoLex-val.tsv | Validation | hard | Tuned | 0.304 |
| Presence | 1_Baseline_0.5_Previous-Sentences-2-val.tsv | Validation | weighted | Tuned | 0.293 |
| Presence | 1_Baseline_0.5_Previous-Sentences-2-val.tsv | Validation | soft | 0.35 | 0.300 |
| Presence | 1_Lex-LIWC-22_LingFeat_0.1_Lex-MJD-val.tsv | Validation | — | 0.50 | 0.294 |
| Presence | ['1_Lex-LIWC-22_LingFeat_0.1_Lex-MJD-val.tsv', '1_Lex-LIWC-22_LingFeat_0.1_Previous-Sentences-2-val.tsv', '1_Lex-LIWC-22_LingFeat_0.1_Lex-eMFD-val.tsv'] | Validation | hard | 0.50 | 0.305 |
| Presence | ['1_Lex-LIWC-22_LingFeat_0.1_Lex-MJD-val.tsv', '1_Lex-LIWC-22_LingFeat_0.1_Previous-Sentences-2-val.tsv', '1_Lex-LIWC-22_LingFeat_0.1_Lex-MFD-20-val.tsv'] | Validation | weighted | 0.50 | 0.307 |
| Presence | ['1_Lex-LIWC-22_LingFeat_0.1_Lex-MJD-val.tsv', '1_Lex-LIWC-22_LingFeat_0.1_Previous-Sentences-2-val.tsv', '1_Lex-LIWC-22_LingFeat_0.1_Lex-eMFD-val.tsv'] | Validation | soft | 0.50 | 0.307 |
| Presence | 1_Lex-LIWC-22_LingFeat_0.1_Lex-MJD-val.tsv | Validation | — | 0.30 | 0.299 |
| Presence | 1_Lex-LIWC-22_LingFeat_0.1_Lex-MJD-val.tsv | Validation | hard | Tuned | 0.299 |
| Presence | ['1_Lex-LIWC-22_LingFeat_0.1_Lex-MJD-val.tsv', '1_Lex-LIWC-22_LingFeat_0.1_Previous-Sentences-2-val.tsv', '1_Lex-LIWC-22_LingFeat_0.1_Lex-MFD-20-val.tsv'] | Validation | weighted | Tuned | 0.307 |
| Presence | 1_Lex-LIWC-22_LingFeat_0.1_Lex-MJD-val.tsv | Validation | soft | 0.40 | 0.299 |

Table S11: Ensemble configurations based on transformer architectures (direct and presence) and the applied filters, and their macro-average F1 on the validation and test sets. Part 2.

| Architecture | Models | Dataset | Mode | Threshold | Macro-F1 |
|---|---|---|---|---|---|
| Presence | 1_Lex-LIWC-22_LingFeat_0.5_Previous-Sentences-2-val.tsv | Validation | — | 0.50 | 0.288 |
| Presence | ['1_Lex-LIWC-22_LingFeat_0.5_Previous-Sentences-2-val.tsv', '1_Lex-LIWC-22_LingFeat_0.5_Baseline-val.tsv'] | Validation | hard | 0.50 | 0.304 |
| Presence | 1_Lex-LIWC-22_LingFeat_0.5_Previous-Sentences-2-val.tsv | Validation | weighted | 0.50 | 0.288 |
| Presence | 1_Lex-LIWC-22_LingFeat_0.5_Previous-Sentences-2-val.tsv | Validation | soft | 0.50 | 0.288 |
| Presence | 1_Lex-LIWC-22_LingFeat_0.5_Lex-MJD-val.tsv | Validation | — | 0.25 | 0.300 |
| Presence | 1_Lex-LIWC-22_LingFeat_0.5_Lex-MJD-val.tsv | Validation | hard | Tuned | 0.300 |
| Presence | 1_Lex-LIWC-22_LingFeat_0.5_Previous-Sentences-2-val.tsv | Validation | weighted | Tuned | 0.288 |
| Presence | ['1_Lex-LIWC-22_LingFeat_0.5_Lex-EmoLex-val.tsv', '1_Lex-LIWC-22_LingFeat_0.5_Previous-Sentences-2-val.tsv', '1_Lex-LIWC-22_LingFeat_0.5_Baseline-val.tsv'] | Validation | soft | 0.25 | 0.308 |
| Presence | 1_Previous-Sentences-2-Lex-eMFD_0.1_Lex-MJD-val.tsv | Validation | — | 0.50 | 0.292 |
| Presence | ['1_Previous-Sentences-2-Lex-eMFD_0.1_Lex-MJD-val.tsv', '1_Previous-Sentences-2-Lex-eMFD_0.1_Previous-Sentences-2-val.tsv'] | Validation | hard | 0.50 | 0.306 |
| Presence | 1_Previous-Sentences-2-Lex-eMFD_0.1_Lex-MJD-val.tsv | Validation | weighted | 0.50 | 0.292 |
| Presence | 1_Previous-Sentences-2-Lex-eMFD_0.1_Lex-MJD-val.tsv | Validation | soft | 0.50 | 0.292 |
| Presence | 1_Previous-Sentences-2-Lex-eMFD_0.1_Lex-MJD-val.tsv | Validation | — | 0.25 | 0.301 |
| Presence | 1_Previous-Sentences-2-Lex-eMFD_0.1_Lex-MJD-val.tsv | Validation | hard | Tuned | 0.301 |
| Presence | 1_Previous-Sentences-2-Lex-eMFD_0.1_Lex-MJD-val.tsv | Validation | weighted | Tuned | 0.292 |
| Presence | ['1_Previous-Sentences-2-Lex-eMFD_0.1_Lex-MJD-val.tsv', '1_Previous-Sentences-2-Lex-eMFD_0.1_Baseline-val.tsv', '1_Previous-Sentences-2-Lex-eMFD_0.1_Previous-Sentences-2-val.tsv'] | Validation | soft | 0.34 | 0.311 |
| Presence | 1_Previous-Sentences-2-Lex-EmoLex_0.1_ResidualBlock-val.tsv | Validation | — | 0.50 | 0.289 |
| Presence | ['1_Previous-Sentences-2-Lex-EmoLex_0.1_ResidualBlock-val.tsv', '1_Previous-Sentences-2-Lex-EmoLex_0.1_Baseline-val.tsv'] | Validation | hard | 0.50 | 0.300 |
| Presence | 1_Previous-Sentences-2-Lex-EmoLex_0.1_ResidualBlock-val.tsv | Validation | weighted | 0.50 | 0.289 |
| Presence | 1_Previous-Sentences-2-Lex-EmoLex_0.1_ResidualBlock-val.tsv | Validation | soft | 0.50 | 0.289 |
| Presence | 1_Previous-Sentences-2-Lex-EmoLex_0.1_Lex-EmoLex-val.tsv | Validation | — | 0.25 | 0.297 |
| Presence | 1_Previous-Sentences-2-Lex-EmoLex_0.1_Lex-EmoLex-val.tsv | Validation | hard | Tuned | 0.297 |
| Presence | 1_Previous-Sentences-2-Lex-EmoLex_0.1_ResidualBlock-val.tsv | Validation | weighted | Tuned | 0.289 |
| Presence | 1_Previous-Sentences-2-Lex-EmoLex_0.1_ResidualBlock-val.tsv | Validation | soft | 0.35 | 0.295 |
| Presence | 1_Previous-Sentences-2-Lex-LIWC-22_0.1_ResidualBlock-val.tsv | Validation | — | 0.50 | 0.292 |
| Presence | ['1_Previous-Sentences-2-Lex-LIWC-22_0.1_ResidualBlock-val.tsv', '1_Previous-Sentences-2-Lex-LIWC-22_0.1_Baseline-val.tsv'] | Validation | hard | 0.50 | 0.301 |
| Presence | ['1_Previous-Sentences-2-Lex-LIWC-22_0.1_ResidualBlock-val.tsv', '1_Previous-Sentences-2-Lex-LIWC-22_0.1_Baseline-val.tsv'] | Validation | weighted | 0.50 | 0.292 |
| Presence | 1_Previous-Sentences-2-Lex-LIWC-22_0.1_ResidualBlock-val.tsv | Validation | soft | 0.50 | 0.292 |
| Presence | 1_Previous-Sentences-2-Lex-LIWC-22_0.1_Lex-EmoLex-val.tsv | Validation | — | 0.30 | 0.299 |
| Presence | 1_Previous-Sentences-2-Lex-LIWC-22_0.1_Lex-EmoLex-val.tsv | Validation | hard | Tuned | 0.299 |
| Presence | ['1_Previous-Sentences-2-Lex-LIWC-22_0.1_ResidualBlock-val.tsv', '1_Previous-Sentences-2-Lex-LIWC-22_0.1_Baseline-val.tsv'] | Validation | weighted | Tuned | 0.292 |
| Presence | 1_Previous-Sentences-2-Lex-LIWC-22_0.1_ResidualBlock-val.tsv | Validation | soft | 0.35 | 0.297 |

Table S12: Ensemble configurations using the best presence models, with macro-average F1 on validation and test sets.

| Models | Dataset | Mode | Threshold | Macro-F1 |
|---|---|---|---|---|
| 1_Lex-LIWC-22_LingFeat_0.1_Lex-MJD-val.tsv | Validation | — | 0.50 | 0.294 |
| ['1_Lex-LIWC-22_LingFeat_0.1_Lex-MJD-val.tsv', '1_Lex-LIWC-22_LingFeat_0.5_Previous-Sentences-2-val.tsv'] | Validation | hard | 0.50 | 0.310 |
| ['1_Lex-LIWC-22_LingFeat_0.1_Lex-MJD-val.tsv', '1_Lex-LIWC-22_LingFeat_0.1_Previous-Sentences-2-val.tsv', '1_Lex-LIWC-22_LingFeat_0.1_Lex-MFD-20-val.tsv'] | Validation | weighted | 0.50 | 0.307 |
| ['1_Lex-LIWC-22_LingFeat_0.1_Lex-MJD-val.tsv', '1_Lex-LIWC-22_LingFeat_0.1_Previous-Sentences-2-val.tsv', '1_Lex-LIWC-22_LingFeat_0.1_Lex-MFD-20-val.tsv'] | Validation | soft | 0.50 | 0.307 |
| 1_Baseline_0.5_Lex-MJD-val.tsv | Validation | — | 0.30 | 0.304 |
| 1_Baseline_0.5_Lex-MJD-val.tsv | Validation | hard | Tuned | 0.304 |
| ['1_Lex-LIWC-22_LingFeat_0.1_Lex-MJD-val.tsv', '1_Lex-LIWC-22_LingFeat_0.1_Previous-Sentences-2-val.tsv', '1_Lex-LIWC-22_LingFeat_0.1_Lex-MFD-20-val.tsv'] | Validation | weighted | Tuned | 0.307 |
| ['1_Baseline_0.5_Lex-MJD-val.tsv', '1_Previous-Sentences-2-Lex-eMFD_0.1_Baseline-val.tsv'] | Validation | soft | 0.31 | 0.312 |
| ['1_Baseline_0.5_Lex-MJD-test.tsv', '1_Previous-Sentences-2-Lex-eMFD_0.1_Baseline-test.tsv'] | Test | — | 0.50 | 0.297 |
| ['1_Baseline_0.5_Lex-MJD-test.tsv', '1_Previous-Sentences-2-Lex-eMFD_0.1_Baseline-test.tsv'] | Test | hard | 0.50 | 0.308 |
| ['1_Baseline_0.5_Lex-MJD-test.tsv', '1_Previous-Sentences-2-Lex-eMFD_0.1_Baseline-test.tsv'] | Test | weighted | 0.50 | 0.291 |
| ['1_Baseline_0.5_Lex-MJD-test.tsv', '1_Previous-Sentences-2-Lex-eMFD_0.1_Baseline-test.tsv'] | Test | soft | 0.50 | 0.291 |
| ['1_Baseline_0.5_Lex-MJD-test.tsv', '1_Previous-Sentences-2-Lex-eMFD_0.1_Baseline-test.tsv'] | Test | — | 0.30 | 0.303 |
| ['1_Baseline_0.5_Lex-MJD-test.tsv', '1_Previous-Sentences-2-Lex-eMFD_0.1_Baseline-test.tsv'] | Test | hard | Tuned | 0.310 |
| ['1_Baseline_0.5_Lex-MJD-test.tsv', '1_Previous-Sentences-2-Lex-eMFD_0.1_Baseline-test.tsv'] | Test | weighted | Tuned | 0.291 |
| ['1_Baseline_0.5_Lex-MJD-test.tsv', '1_Previous-Sentences-2-Lex-eMFD_0.1_Baseline-test.tsv'] | Test | soft | 0.31 | 0.318 |

Table S13: Ensemble configurations using the final best direct and presence models, with macro-average F1 on validation and test sets.

| Models | Dataset | Mode | Threshold | Macro-F1 |
|---|---|---|---|---|
| direct_champion-tuned-soft-champion-val.tsv | Validation | — | 0.50 | 0.291 |
| ['direct_champion-tuned-soft-champion-val.tsv', 'presence_champion-tuned-soft-champion-val.tsv'] | Validation | hard | 0.50 | 0.315 |
| direct_champion-tuned-soft-champion-val.tsv | Validation | weighted | 0.50 | 0.291 |
| direct_champion-tuned-soft-champion-val.tsv | Validation | soft | 0.50 | 0.291 |
| direct_champion-tuned-soft-champion-val.tsv | Validation | — | 0.30 | 0.326 |
| direct_champion-tuned-soft-champion-val.tsv | Validation | hard | Tuned | 0.326 |
| direct_champion-tuned-soft-champion-val.tsv | Validation | weighted | Tuned | 0.291 |
| direct_champion-tuned-soft-champion-val.tsv | Validation | soft | 0.29 | 0.326 |
| direct_champion-tuned-soft-champion-test.tsv | Test | — | 0.50 | 0.287 |
| direct_champion-tuned-soft-champion-test.tsv | Test | hard | 0.50 | 0.287 |
| direct_champion-tuned-soft-champion-test.tsv | Test | weighted | 0.50 | 0.287 |
| direct_champion-tuned-soft-champion-test.tsv | Test | soft | 0.50 | 0.287 |
| direct_champion-tuned-soft-champion-test.tsv | Test | — | 0.30 | 0.328 |
| direct_champion-tuned-soft-champion-test.tsv | Test | hard | Tuned | 0.328 |
| direct_champion-tuned-soft-champion-test.tsv | Test | weighted | Tuned | 0.287 |
| direct_champion-tuned-soft-champion-test.tsv | Test | soft | 0.29 | 0.332 |

Table S14: LLM Ensemble configurations, with macro-average F1 on validation and test sets.

| **Models** | **Dataset** | **Mode** | **Threshold** | **Macro-F1** |
|---|---|---|---|---|
| ['definition-20/google-gemma-2-9b-it-gated_Presence-val.tsv', 'qlora-direct-lr-2e-4/google-gemma-2-9b-it-val.tsv'] | Validation | hard | 0.50 | 0.275 |
| definition-20/google-gemma-2-9b-it-gated_Presence-val.tsv | Validation | weighted | 0.50 | 0.232 |
| ['definition-20/google-gemma-2-9b-it-gated_Presence-val.tsv', 'qlora-direct-lr-2e-4/google-gemma-2-9b-it-val.tsv'] | Validation | soft | 0.50 | 0.275 |
| ['definition-20/google-gemma-2-9b-it-gated_Presence-test.tsv', 'qlora-direct-lr-2e-4/google-gemma-2-9b-it-test.tsv'] | Test | hard | 0.50 | 0.277 |
| ['definition-20/google-gemma-2-9b-it-gated_Presence-test.tsv', 'qlora-direct-lr-2e-4/google-gemma-2-9b-it-test.tsv'] | Test | weighted | 0.50 | 0.238 |
| ['definition-20/google-gemma-2-9b-it-gated_Presence-test.tsv', 'qlora-direct-lr-2e-4/google-gemma-2-9b-it-test.tsv'] | Test | soft | 0.50 | 0.277 |

Table S15: Hybrid Ensemble configurations, with macro-average F1 on validation set.

| **Models** | **Dataset** | **Mode** | **Threshold** | **Macro-F1** |
|---|---|---|---|---|
| direct_champion-tuned-soft-champion-val.tsv | Validation | hard | 0.50 | 0.291 |
| ['direct_champion-tuned-soft-champion-val.tsv', 'llm/fixed-hard-champion-val.tsv'] | Validation | weighted | 0.50 | 0.313 |
| direct_champion-tuned-soft-champion-val.tsv | Validation | soft | 0.50 | 0.291 |
| direct_champion-tuned-soft-champion-val.tsv | Validation | hard | Tuned | 0.326 |
| ['direct_champion-tuned-soft-champion-val.tsv', 'llm/fixed-hard-champion-val.tsv'] | Validation | weighted | Tuned | 0.320 |
| ['direct_champion-tuned-soft-champion-val.tsv', 'llm/fixed-hard-champion-val.tsv'] | Validation | soft | 0.53 | 0.319 |

Table S16: Transformer models statistical tests with McNemar test $p$-values. “Setup” concatenates Type, Architecture, Name, threshold (Thr.), filter model (Filter) and filter threshold (Filt. Thr.). “Comp.” indicates the type of comparison, ΔF1 LB is the one-sided lower 95% bound on the F1 difference (Model2–Model1), and “Sig.” indicates whether the comparison is statistically significant under the chosen criterion.

| Setup | V1 | V2 | V3 | V4 | V5 | V6 | V7 | V8 | V9 | V10 | V11 | V12 | V13 | V14 | V15 | V16 | V17 | V18 | V19 | Macro-F1 | Comp. | ΔF1 LB | p(Model2>1) | Sig. |
|---|---|---|---|---|---|---|---|---|---|---|---|---|---|---|---|---|---|---|---|---|---|---|---|---|
| Arch.: Direct. Name: Lex – LIWC 22. Thr.: 0.50. Filter: None | — | — | — | — | — | — | — | — | — | — | — | — | — | — | — | — | — | — | — | 0.286 | Model | -0.002 | 0.144 | No |
| Arch.: Direct. Name: Baseline. Thr.: 0.30. Filter: None | 0.00 | 0.00 | 0.00 | 0.02 | 0.00 | 0.00 | 0.00 | 0.00 | 0.00 | 0.00 | 0.00 | 0.00 | 0.00 | 1.00 | 0.00 | 0.00 | 0.00 | 0.00 | 0.00 | 0.311 | Tuning threshold | 0.023 | 0.000 | Yes |
| Arch.: Direct. Name: Lex – LIWC 22. Thr.: 0.25. Filter: None | — | — | — | — | — | — | — | — | — | — | — | — | — | — | — | — | — | — | — | 0.320 | Tuning threshold + Model | -0.001 | 0.073 | No |
| Arch.: Presence. Name: Lex – MJD. Thr.: 0.50. Filter: Previous-Sentences-2-Lex-LIWC-22. Filt. Thr.: 0.10 | 1.00 | 0.05 | 0.60 | 0.43 | 0.00 | 1.00 | 1.00 | 1.00 | 0.73 | 0.60 | 1.00 | 0.60 | 0.69 | — | 0.01 | 0.06 | 0.64 | 1.00 | 0.43 | 0.303 | Model | 0.004 | 0.005 | Yes |
| Arch.: Presence. Name: Baseline. Thr.: 0.30. Filter: Previous-Sentences-2-Lex-LIWC-22. Filt. Thr.: 0.10 | 0.00 | 0.00 | 0.00 | 0.13 | 0.00 | 0.00 | 0.00 | 0.00 | 0.00 | 0.00 | 0.00 | 0.00 | 0.03 | 0.00 | 0.00 | 0.00 | 0.00 | 0.00 | 0.00 | 0.303 | Tuning threshold | 0.006 | 0.000 | Yes |
| Arch.: Presence. Name: Lex – MJD. Thr.: 0.40. Filter: Previous-Sentences-2-Lex-LIWC-22. Filt. Thr.: 0.10 | 0.39 | 0.56 | 0.42 | 0.14 | 0.01 | 0.15 | 0.02 | 0.14 | 0.04 | 0.00 | 0.32 | 0.14 | 0.33 | 1.00 | 0.46 | 0.48 | 0.01 | 0.14 | 0.82 | 0.313 | Tuning threshold + Model | 0.002 | 0.020 | Yes |
| Arch.: Presence. Name: Lex – MJD. Thr.: 0.40. Filter: Previous-Sentences-2-Lex-LIWC-22. Filt. Thr.: 0.10 | — | — | — | — | — | — | — | — | — | — | — | — | — | — | — | — | — | — | — | 0.313 | Architecture champions | -0.006 | 0.392 | No |
| Arch.: Ensemble Transformer. Name: direct_champion-tuned-soft-champion-test.tsv. Thr.: 0.29. Filter: None | 1.00 | 0.00 | 0.11 | 0.54 | 0.93 | 0.00 | 0.02 | 0.01 | 0.00 | 0.00 | 0.04 | 0.00 | 0.30 | 1.00 | 0.66 | 0.06 | 0.01 | 0.06 | 0.30 | 0.332 | Single vs. Ensemble Transformer champions | 0.012 | 0.000 | Yes |

Table S17: LLM statistical tests with McNemar test $p$-values. "Setup" concatenates Type, Architecture, Name, threshold (Thr.), filter model (Filter) and filter threshold (Filt. Thr.). "Comp." indicates the type of comparison, $\Delta$F1 LB is the one-sided lower 95% bound on the F1 difference (Model2–Model1), and "Sig." indicates whether the comparison is statistically significant under the chosen criterion.

| **Setup** | **V1** | **V2** | **V3** | **V4** | **V5** | **V6** | **V7** | **V8** | **V9** | **V10** | **V11** | **V12** | **V13** | **V14** | **V15** | **V16** | **V17** | **V18** | **V19** | **Macro-F1** | **Comp.** | **$\Delta$F1 LB** | **p(Model2>1)** | **Sig.** |
|---|---|---|---|---|---|---|---|---|---|---|---|---|---|---|---|---|---|---|---|---|---|---|---|---|
| Arch.: Direct. Name: Gemma 2 9B Zero-Shot hier (SBERT gate). Thr.: —. Filter: SBERT gate. Filt. Thr.: 0.29 | 0.16 | 0.02 | 0.00 | 0.05 | 0.00 | 0.28 | 0.03 | 0.28 | 0.00 | 0.00 | 0.03 | 0.00 | 0.16 | 1.00 | 0.53 | 1.00 | 0.16 | 0.00 | 1.00 | 0.229 | Adding SBERT gate | 0.005 | 0.000 | Yes |
| Arch.: Direct. Name: Gemma 2 9B Few-Shot. Thr.: —. | 0.51 | 0.01 | 0.02 | 0.02 | 0.10 | 0.08 | 0.64 | 0.00 | 0.00 | 0.64 | 0.00 | 1.00 | 0.01 | 0.01 | 1.00 | 0.00 | 0.02 | 0.10 | 0.10 | 0.00 | Zero-Shot vs. Few-Shot | 0.005 | 0.001 | Yes |
| Arch.: Direct. Name: Gemma 2 9B Few-Shot hier (SBERT gate). Thr.: —. Filter: SBERT gate. Filt. Thr.: 0.29 | 0.09 | 0.00 | 0.00 | 0.02 | 0.00 | 0.16 | 0.03 | 0.57 | 0.00 | 0.00 | 0.09 | 0.00 | 0.09 | 1.00 | 0.30 | 1.00 | 1.00 | 0.00 | 1.00 | 0.238 | Adding SBERT gate | 0.003 | 0.000 | Yes |
| Arch.: Direct. Name: Gemma 2 9B Few-Shot hier (SBERT gate). Thr.: —. Filter: SBERT gate. Filt. Thr.: 0.29 | — | — | — | — | — | — | — | — | — | — | — | — | — | — | — | — | — | — | — | 0.238 | Finetuning with QLoRA vs. Best zero/few-shot | -0.010 | 0.386 | No |
| Arch.: Ensemble of LLM. Name: fixed-hard-champion-test.tsv. Thr.: —. Filter: None | 0.32 | 0.00 | 0.00 | 0.01 | 0.00 | 0.00 | 0.00 | 0.00 | 0.00 | 0.00 | 0.00 | 0.00 | 0.59 | 1.00 | 0.00 | 0.00 | 1.00 | 0.32 | 1.00 | 0.277 | Single vs. Ensemble LLM | 0.034 | 0.000 | Yes |
| Arch.: Direct. Name: direct_champion-tuned-soft-champion-test.tsv. Thr.: 0.29. Filter: None | 0.24 | 1.00 | 0.00 | 0.80 | 0.00 | 0.00 | 0.67 | 0.93 | 0.01 | 0.00 | 0.00 | 0.03 | 0.28 | 1.00 | 0.00 | 0.00 | 0.07 | 0.04 | 0.97 | 0.332 | Transformer vs. LLM champions | 0.045 | 0.000 | Yes |
